# Supplementary material for: A statistical network analysis of the HIV/AIDS epidemics in Cuba
Source: arXiv:1401.6449 source file (2015-05-22)
Supplement: Supplementary file 1 [file suppl-material-v3.pdf]

# Supplementary materials for "A statistical network analysis of the HIV/AIDS epidemics in Cuba"

Stéphan Clémençon, Hector De Arazoza, Fabrice Rossi, Viet Chi Tran

May 20, 2015

## Contents

**1 Background** 1

**2 Descriptive statistics** 2
- 2.1 Sexual orientation . . . 2
- 2.2 Geographical location . . . 3
- 2.3 Age at detection . . . 3

**3 Detection method** 4
- 3.1 Time evolution . . . 5
- 3.2 Efficiency of contact-tracing described by mean of the other covariates . . . 5
- 3.3 Should we study the contacts of individuals detected by contact-tracing ? . . . 6

**4 Infection tree** 9

**5 Degree distribution** 10
- 5.1 Covariate description . . . 11
- 5.2 Calibration of power-law distributions . . . 11
  - 5.2.1 Minization Küllback-Leibler divergence . . . 11
  - 5.2.2 Hill estimator of the power . . . 14
- 5.3 Prediction of the appearance of the giant component . . . 14
- 5.4 Isolated individuals . . . 15

**6 Statistical summary of the graph** 16
- 6.1 Assortative mixing coefficients . . . 16
- 6.2 Clustering properties . . . 16
  - 6.2.1 Clustering coefficients . . . 16
  - 6.2.2 Global path length . . . 18
- 6.3 Network resilience, shortest-path centrality . . . 18

**7 Study of the giant component** 20
- 7.1 Covariate distribution . . . 20
- 7.2 Supplementary material for the clustering of the giant component . . . 20
- 7.3 The 37 clusters of the giant component . . . 22

# 1 Background

As describe in the body of the article [4], a contact-tracing detection system has been set up in Cuba since 1986 to bring the spread of the AIDS-HIV epidemics under control. The contact-tracing system has enabled to collect and gather a considerable amount of epidemiological data, very detailed at the individual level, though anonymous. The database is constituted of 5,389 individual tested as HIV positive and described through several attribute variables: year and age of detection, gender and sexual orientation, detection mode, province of residence, identifier of the infecting contact, number of sexual partners in the last two years, number of partners tested for HIV and number of infected partners.

It is estimated that because the number of tests is high and because the central laboratory applies specific tests in case of uncertain results, there is no false positive/negative cases. More precisely, the detection system is based on multiple testing. If a person, that is the contact of a known HIV+, tests negative in a first test, the person is tested

at least 2 more times to be certain that HIV is not present in his/her system. If a person tests positive to HIV , more tests (specific to HIV) are performed to ensure that it is not a false positive.
Additionally, a list of indices corresponding to the sexual partners appearing in the database she/he possibly named for contact-tracing is also available. In many situations, a medical investigation enabled to provide in addition a plausible date of infection, together with the index of the supposed HIV transmitter.

This provides a graph, where the vertices represent the individuals detected as HIV positive between 1986 and 2006. The individuals tested HIV negative and declared as sexual contacts of the latter are not recorded in the database and thus, do not enter the study. The 5,389 individuals in the database are linked by 4,073 edges. Upon detection, when an individual names her/his sexual partners during the two previous years for contact-tracing, new infectious individuals are detected and added to the database. Edges between them and the individual who gave their names indicate the detection graph and the fact that they have been sexual partners. These edges are *directed* and running from the individual who provided the contact information (*Ego* of the directed edge) to the detected one (*Alter* of the edge). When it is considered true that one individual has infected another one, the related information is incorporated by considering a directed edge pointing in the direction of probable HIV transmission. The graph representing the HIV transmissions naturally correspond to subtrees of this network.

We have a very rich graph exhibiting a giant component constituted of 2,386 individuals (44.28% of the graph vertices) and 3,168 edges (77.78% of the graph edges), which is very rare in social networks studies (see *e.g.* in [10, 12] where the giant components are of sizes 82 and 965 out of 4,544 and 2,200 individuals respectively). As for various real-world networks, it is much larger than the size of the second largest component, here 17 for the second largest component see Table 1 (see section IV A in[9] and the references therein).

| Component size | 1 | 2 | 3 | 4 | 5 | 6 | 7 | 8 | 9 | 10 | 11 | 13 | 14 | 17 | 2,386 |
|---|---|---|---|---|---|---|---|---|---|---|---|---|---|---|---|
| Number of component | 1,627 | 308 | 88 | 36 | 22 | 12 | 5 | 4 | 2 | 3 | 1 | 1 | 1 | 1 | 1 |

Table 1: *Sizes of the connected components of the sexual contact network.*

In Section 2, we provide summary statistics for the covariates characterizing the individuals of our database (sexual orientation, geographical location and age at detection). The detection source and its efficiency are analyzed in Section 3. This is refined by exploration of the infection tree in Section 4. The degree distributions of the graph are carefully considered in Section 5 and summary statistics describing the network are computed in Section 6. In Section 7 we provide additional figures and tables that complement the description in the main text.

# 2 Descriptive statistics

We start by giving figures for the variables 'sexual orientation', 'geographical location' and 'age at detection'. The method of detection and the covariates describing degree distributions are studied separately.

## 2.1 Sexual orientation

The variables 'gender' and 'sexual orientation' can be merged, insofar as they stratify the population in only three categories, relevant for the present analysis (sexual transmission of HIV between women being neglected): women, heterosexual men and Men having Sex with Men (MSM, in the sequel).

| | Woman | Heterosexual man | MSMl |
|---|---|---|---|
| Frequency | 1,109 | 566 | 3,714 |
| Proportion | 20.58% | 10.50% | 68.92% |

Table 2: *Distribution of sexual orientation.*

As we see, the disease appears at first sight as highly bisexual (68.92%). However, the evolution of the number of HIV-AIDS individuals per sexual orientation (see Fig. 1) reveals that the very epidemics may have been first heterosexual before reaching women and MSMs. A first outbreak is observed around 1991. In 1993-1994, a decrease in detections is seen, which may be due to the economic crisis following the collapse of the Soviet Union. Then, a large increase of the epidemics is observed beginning in 1995. The analysis of the clusters in the giant component will later provide some additional information on the evolution of the disease (see also [3]).

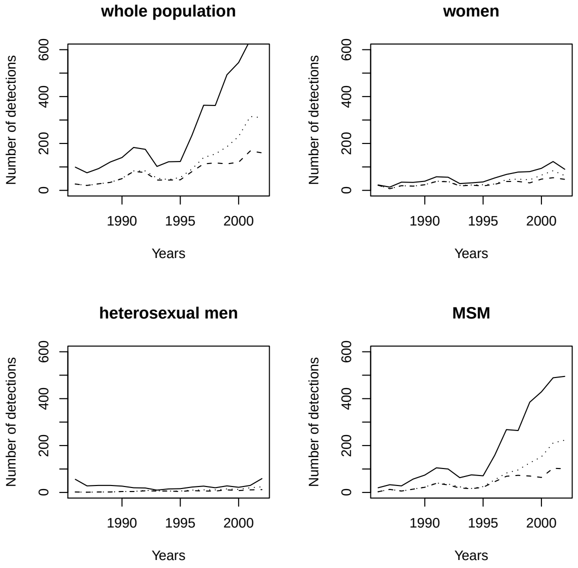


Figure 1: *Evolution of the epidemics in the whole population and per sexual orientation.*

## 2.2 Geographical location

For the geographical location, the island being divided into four regions, as depicted by Fig. 2. Since 53.48% of the detected seropositive individuals live in the *Ciudad de La Havana* (modality 'CH' of the variable 'area of residence'), the city is often considered apart.

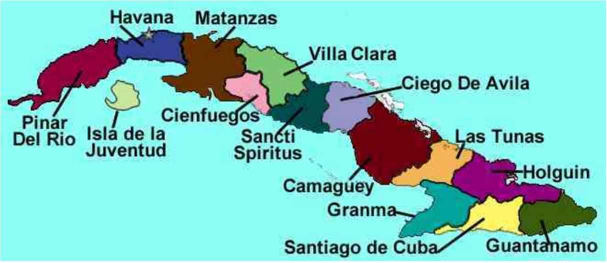


Figure 2: *Provinces of Cuba. West: Pinar Del Rio, Isla de la Juventud, Matanzas. Central: Cienfuegos, Villa Clara, Sancti Spiritus. East-Central: Ciego De Avila, Camaguey, Las Tunas. East: Holguin, Granma, Santiago de Cuba, Guantanamo. The City and province of La Havana are considered as the fifth area.*

| | West | Central | East-Central | East | La Havana |
|---|---|---|---|---|---|
| Frequency | 468 | 829 | 337 | 645 | 3,110 |
| Proportion (%) | 8.68 | 15.38 | 6.25 | 11.97 | 57.71 |

Table 3: *Distribution by geographic location.*

## 2.3 Age at detection

Age of newly infected individuals is slightly increasing through years, with a larger variance (Fig. 3 (b)). The mean age at detection is 29.43 year old and it is lower for women and individuals detected by contact-tracing (see Tables 4 and 5) although the stratifications by sexual orientation or detection method are not significant according to ANOVA tests.

| Age class | [10,20) | [20,30) | [30,40) | [40,50) | [50,90) |
|---|---|---|---|---|---|
| Frequency | 580 | 2,403 | 1,625 | 508 | 185 |

Table 4: *Age distribution at detection. Only the individuals which were infected after 10 years old are being considered (5,301 individuals).*

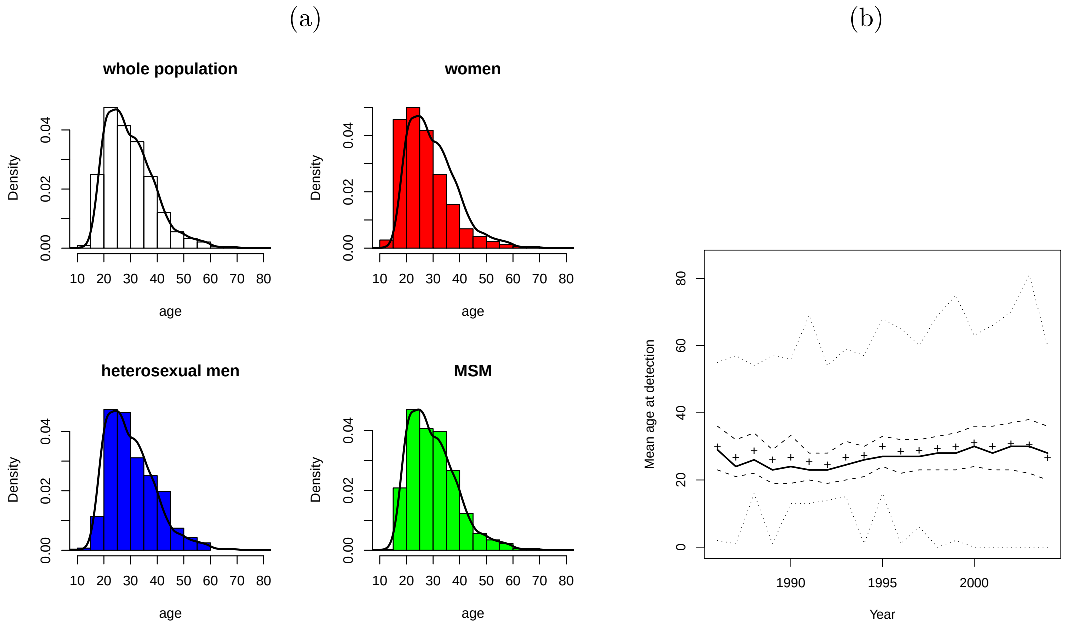


Figure 3: *(a): Histogram for the age at detection, by sexual orientation. (b): Evolution of the age at detection. Yearly statistics are computed. In plain line is the median age at detection. The crosses correspond to the means. In dashed lines are the first and third quartiles. The minima and maxima stand in dotted line. The linear regression of age at detection* $Y$ *on year of detection* $X$ *gives:* $Y = -496.88 + 0.26X$. *Although the regression has a low* $R^2_{adj} = 1.54\%$, *the Fisher test tells that it is statistically significant.*

| Age at detection | Mean | Std. dev. | Min | Max | Median |
|---|---|---|---|---|---|
| Whole population | 29.43 | 9.13 | 11 | 81 | 28 |
| La Havana | 30.71 | 9.30 | 12 | 81 | 30 |
| Women | 26.78 | 9.10 | 12 | 81 | 25 |
| Heterosexual men | 31.07 | 9.00 | 11 | 59 | 29 |
| MSM | 29.98 | 9.01 | 13 | 75 | 29 |
| CONTA | 27.71 | 8.81 | 12 | 81 | 26 |
| CAPTA | 31.17 | 10.03 | 14 | 67 | 30 |
| RANDOM | 29.82 | 8.91 | 11 | 75 | 28 |

Table 5: *Age distribution at detection. Only the individuals which were infected after 6 years old are being considered (5,303 individuals).*

# 3 Detection method

Special attention is paid to the variable 'detection type', indicating the way of detection, which counts three modalities: 'CONTA' when the individual has been detected by means of contact-tracing, 'CAPTA' if detection has occurred as a result of a visit to the family doctor, which we call captation, and 'RANDOM' for a detection due to the (random) screening-based detection system (see Table 6).

| | CONTA | CAPTA | RANDOM |
|---|---|---|---|
| Frequency | 1,515 | 821 | 3,053 |
| Proportion | 28.11% | 15.23% | 56.65% |

Table 6: *Repartition by method of detection.*

## 3.1 Time evolution

We see on Fig. 4 that there is a burst in the epidemics (observable through the burst in the number of detections) starting in 1995. Due to limited capacity of information treatment, the contact-tracing system does not follow. However, if we include the captation detections by intermediary of the doctors to the contact-tracing detections, we see that about one half of the detections are due to non-random methods as is shown in Table 7. This results confirm the figures in [2, 5], where statistical analysis showed that in the last years contact-tracing and captation methods accounted for almost one detection out of two. The role of contact-tracing can also be seen when comparing the distribution of detection method in the whole population, for isolated individuals and in the giant component (Tables 19): non-random methods account for 43.35% of the detection in the whole population, whereas they represent 50.71% of the detection in the largest component and 25.32% of the detection for isolated individuals.

| | 2000 | 2001 | 2002 | 2003 | 2004 | Total |
|---|---|---|---|---|---|---|
| Non-random | 42.2% | 49.1% | 48.1% | 50.9% | 39.4% | 47.5% |
| Contact-tracing only | 22.0% | 26.2% | 24.8% | 22.7% | 19.7% | 23.8% |

Table 7: *Percentage of detections due to non-random methods and contact-tracing over the last years. The data for the last year are not complete which explains the apparent decrease in the figures.*

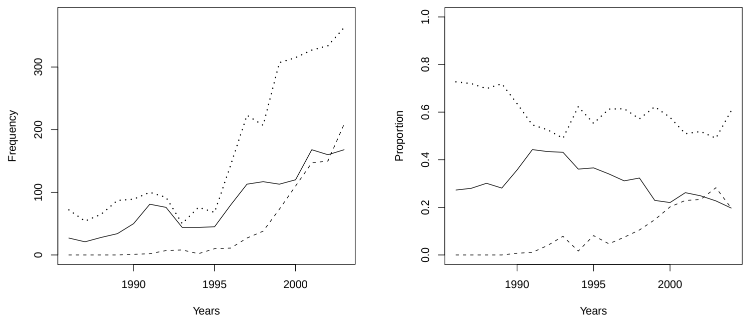


Figure 4: *Evolution of the number of detections via contact-tracing (plain line), captation (dashed line) and random methods (dotted line).*

## 3.2 Efficiency of contact-tracing described by mean of the other covariates

At first glance, the predominance of “nonrandom detection methods” (i.e. detections by contact-tracing or captation) appears clearly: the latter account for 65.5%, 33.5% and 38.2% of the detections for women, heterosexual men and MSM respectively. A $\chi^2$-test reveals that the variables 'gender/sexual orientation' and 'way of detection' are not independent, even if one restricts the population under study to a specific area: $p$-values are smaller than $10^{-16}$. The strong departure from independence is due to the following facts. 1) more women are detected by means of contact-tracing than by random detections, 2) more men are detected through random detections than by means of contact-tracing. 3) detections by captation act equally whatever the sexual orientation.

The different detection methods are represented differently in the five geographical regions of our study, as shown in Table 9. Deviations to independence are essentially due to the West and Central areas and to La Havana. The city of La Havana is characterized by a higher percentage of random detections and a lower percentage of detections *via* contact-tracing, while this is the reverse in the West and Central areas.

We see that the contact-tracing detection is mostly efficient for women and in the West and Central areas. In return, we will see in Table 11 that women, for instance, contribute most to finding new infectious individuals, once they have been detected (29.66%).

| | CONTA | CAPTA | RANDOM | Total |
|---|---|---|---|---|
| Women | 573 (51.7%,37.8%)<br>*312* | 153 (13.8%,18.6%)<br>*169* | 383 (34.5%,12.5%)<br>*628* | 1,109 |
| Heterosexual men | 124 (21.9%,8.2%)<br>*159* | 66 (11.7%,8.0%)<br>*86* | 376 (66.4%,12.3%)<br>*321* | 566 |
| MSM | 818 (22.0%,54.0%)<br>*1,044* | 602 (16.2%,73.3%)<br>*566* | 2,294 (61.8%,75.1%)<br>*2,104* | 3,714 |
| Total | 1,515 | 821 | 3,053 | 5,389 |

Table 8: *Contingency table describing the relation between the categorical variables 'gender/sexual orientation' and 'way of detection'. Expected sizes under the assumption of independence are given in italic script, between the brackets, row and column percentages are respectively given. Strong dependence is shown (*p*-value of* $\chi^2$*-test is smaller than* $10^{-16}$*): 65.5% (resp. 33.6% and 38.2%) of the women (resp. of heterosexual men and MSM) are detected by non-random detection methods (CONTA and CAPTA).*

| | CONTA | CAPTA | RANDOM | Total |
|---|---|---|---|---|
| West | 187 (40.0%,12.3%)<br>*132* | 66 (14.1%,8.0%)<br>*71* | 215 (45.9%,7.0%)<br>*265* | 468 |
| Central | 341 (41.1%,22.5%)<br>*233* | 89 (10.7%,10.8%)<br>*126* | 399 (48.1%,13.1%)<br>*470* | 829 |
| East-Central | 86 (25.5%,5.7%)<br>*95* | 55 (16.3%,6.7%)<br>*51* | 196 (58.2%,6.4%)<br>*191* | 337 |
| East | 197 (30.5%,13.0%)<br>*181* | 102 (15.8%,12.4%)<br>*98* | 346 (53.6%,11.3%)<br>*365* | 645 |
| La Havana | 704 (22.6%,46.5%)<br>*874* | 509 (16.4%,62.0%)<br>*474* | 1,897 (61.0%,62.1%)<br>*1,762* | 3,110 |
| Total | 1,515 | 821 | 3,053 | 5,389 |

Table 9: *Contingency table describing the relation between 'geographical location' and 'way of detection'. Expected sizes under the assumption of independence are given in italic script, between the brackets, row and column percentages are respectively given. Strong dependence is shown:* p*-value of* $\chi^2$*-test equals* $2.2\,10^{-16}$

If we restrict to La Havana, which corresponds to 3110 individuals, we find the Table 10:

| | CONTA | CAPTA | RANDOM | Total |
|---|---|---|---|---|
| Women | 206 (43.7%,29.3%)<br>*107* | 61 (13.0%,12.0%)<br>*77* | 204 (43.3%,10.8%)<br>*287* | 471 |
| Heterosexual men | 34 (16.4%,4.8%)<br>*47* | 35 (16.9%,6.9%)<br>*34* | 138 (66.7%,7.3%)<br>*126* | 207 |
| MSM | 464 (19.1%,65.9%)<br>*551* | 413 (17.0%,81.1%)<br>*398* | 1,555 (63.9%,82.0%)<br>*1,483* | 2,432 |
| Total | 704 | 509 | 1,897 | 3,110 |

Table 10: *Contingency table describing the relation between the categorical variables 'gender/sexual orientation' and 'way of detection' for La Havana. Expected sizes under the assumption of independence are given in italic script, between the brackets, row and column percentages are respectively given. Strong dependence is shown (*p*-value of* $\chi^2$*-test equals* $2.2\,10^{-16}$*): 56.7% (resp. 33.3% and 36%) of the women (resp. of heterosexual men and MSM) are detected by non-random detection methods (CONTA and CAPTA).*

### 3.3 Should we study the contacts of individuals detected by contact-tracing ?

We consider this question which has already been tackled by [7] by mean of a sophisticated compartmental model. When an individual gives her/his contacts, in average, 76.89% of the latter are tested (median of 84.62%) and 22.52% of the contacts given by an individual are tested positive (median of 14.29%) (see Table 11). The proportion of tested (resp. detected positive) contacts for egos who have been detected by contact-tracing is 80.91% (resp. 34.15%) which is higher than the proportion for the whole population (76.89% resp. 22.52%) or for egos detected by random methods (76.29% resp. 18.57%). This probably comes from the fact that people detected by contact-tracing may have a larger

degree than other individuals.

| Variable | Mean | Standard deviation | Minimum | Maximum | Median |
|---|---|---|---|---|---|
| Whole population | | | | | |
| Number of contacts | 6.17 | 5.54 | 1 | 82 | 5 |
| Nb. of tested contacts | 4.75 | 4.88 | 0 | 74 | 3 |
| Nb. of detected positive contacts | 1.04 | 1.31 | 0 | 19 | 1 |
| Prop. of tested contacts | 76.89% | 27.06% | 0 | 100% | 84.62% |
| Prop. of detected positive contacts | 22.52% | 27.57% | 0 | 100% | 14.29% |
| Prop. of contacts in the graph | 14.56% | 23.01% | 0 | 100% | 0 |
| Ego is detected by contact-tracing | | | | | |
| Nb. of contacts | 6.43 | 5.39 | 1 | 54 | 5 |
| Nb. of tested contacts | 5.11 | 4.64 | 0 | 37 | 4 |
| Nb. of detected positive | 1.56 | 1.45 | 0 | 14 | 1 |
| Prop. of tested | 80.91% | 25.22% | 0 | 100% | 91.67% |
| Prop. of detected positive | 34.15% | 29.49% | 0 | 100% | 25% |
| Prop. of contacts in the graph | 14.54% | 21.48% | 0 | 100% | 0 |
| Ego is detected by captation | | | | | |
| Nb. of contacts | 6.07 | 5.04 | 1 | 62 | 5 |
| Nb. of tested contacts | 4.36 | 4.27 | 0 | 38 | 3 |
| Nb. of detected positive | 0.65 | 0.92 | 0 | 8 | 0 |
| Prop. of tested | 71.24% | 29.30% | 0 | 100% | 75 |
| Prop. of detected positive | 14.18% | 22.31% | 0 | 100% | 0 |
| Prop. of contacts in the graph | 11.79% | 21.78% | 0 | 100% | 0 |
| Ego is detected by random methods | | | | | |
| Nb. of contacts | 6.06 | 5.75 | 1 | 82 | 5 |
| Nb. of tested contacts | 4.67 | 5.14 | 0 | 74 | 3 |
| Nb. of detected positive | 0.87 | 1.24 | 0 | 19 | 1 |
| Prop. of tested | 76.29% | 27.05% | 0 | 100% | 83.33% |
| Prop. of detected positive | 18.57% | 25.83% | 0 | 100% | 8.33% |
| Prop. of contacts in the graph | 15.33% | 24.05% | 0 | 100% | 0 |
| Ego is a woman | | | | | |
| Nb. of contacts | 5.89 | 5.03 | 1 | 39 | 5 |
| Nb. of tested contacts | 4.82 | 4.49 | 0 | 37 | 4 |
| Nb. of detected positive | 1.20 | 1.30 | 0 | 9 | 1 |
| Prop. of tested | 82.26% | 25.43% | 0 | 100% | 100% |
| Prop. of detected positive | 29.66% | 30.28% | 0 | 100% | 20 |
| Prop. of contacts in the graph | 9.76% | 18.37% | 0 | 100% | 0 |
| Ego is a heterosexual man | | | | | |
| Nb. of contacts | 4.98 | 4.11 | 1 | 30 | 4 |
| Nb. of tested contacts | 3.96 | 3.59 | 0 | 27 | 3 |
| Nb. of detected positive | 0.73 | 1.08 | 0 | 11 | 0 |
| Prop. of tested | 83.22% | 25.91% | 0 | 100% | 100% |
| Prop. of detected positive | 19.50% | 28.44% | 0 | 100% | 0 |
| Prop. of contacts in the graph | 15.36% | 25.95% | 0 | 100% | 0 |
| Ego is a MSM | | | | | |
| Nb. of contacts | 6.43 | 5.84 | 1 | 82 | 5 |
| Nb. of tested contacts | 4.85 | 5.14 | 0 | 74 | 4 |
| Nb. of detected positive | 1.04 | 1.34 | 0 | 19 | 1 |
| Prop. of tested | 74.31% | 27.32% | 0 | 100% | 80% |
| Prop. of detected positive | 20.73% | 26.16% | 0 | 100% | 12.50% |
| Prop. of contacts in the graph | 15.94% | 23.65% | 0 | 100% | 0 |

Table 11: *Summary statistics for the number of declared contacts 'ncontact', the proportion of tested contacts ('ncon-ttest/ncontact'), the proportion of positive contacts ('ncontpos/ncontact') and the proportion of positive contacts in the graph ('number of contacts in the graph/ncontact') for the whole population and according to various co-variates. We exclude from the analysis the individuals for whom the number of contacts is missing. The proportion of positive contacts in the graph takes into account the fact that when a new infected gives his contacts, some have already been detected before.*

In Table 12, we compare the detection methods for alters whose egos have been detected by contact-tracing or random screening. A $\chi^2$-test accepts the adequation with p-value of 11.86%. All the same, when considering random and non-random detection methods (by gathering contact-tracing and captation), adequation is accepted with a p-value of 6.12%. As a consequence, investigating the contacts of infectious individuals detected by contact-tracing does not seem to be less efficient than considering the contacts of individuals detected by random screenings.

| | Alter is CONTA | Alter is CAPTA | Alter is RANDOM | Total |
|---|---|---|---|---|
| Ego is CONTA | 578 (35.35%,34.30%) | 157 (9.60%, 29.79%) | 900 (55.05%,30.72%) | 1,635 (*31.80%*) |
| Ego is CAPTA | 180 (27.27%,10.68%) | 106 (16.06%,20.11%) | 374 (56.67%,12.77%) | 660 (*12.84%*) |
| Ego is RANDOM | 927 (32.57%,55.01%) | 264 (9.28,50.09%) | 1,655 (58.15%,56.50%) | 2,846 (*55.36%*) |
| Total | 1,685 (*32.78%*) | 527 (*10.25%*) | 2,929 (*56.97%*) | |

Table 12: *Type of detection of egos and alters for the edges in the detection graph.*

To have a further idea of how the non-random detections help the health system to extract new infectious individuals, let us investigate the times separating an ego from its alters. Times of detection along one edge are shown to be shorter for edges with ego detected by non-random method (see Tables 13 and 14) when compared to ego detected by random methods. The results are presented in Table 13 and seem to show that non-random methods help a more rapid detection of unknown infectious seropositives. To check that these differences are not related to the fact that individuals detected by non-random methods belong to clusters that are being actively explored, we also compute the mean time needed to find a contact among the edges that have actually serve for contact-tracing detection.

| Variable | Mean | Standard deviation | Minimum | Maximum | Median |
|---|---|---|---|---|---|
| Whole population | 686.66 | 837.56 | 1 | 5,768 | 344 |
| Ego is CONTA | 698.79 | 854.32 | 1 | 5,435 | 344 |
| Ego is CAPTA | 428.39 | 520.76 | 1 | 3,683 | 238 |
| Ego is RANDOM | 725.64 | 865.08 | 1 | 5,768 | 386 |
| Ego is woman | 725.64 | 937.37 | 1 | 5,364 | 309 |
| Ego is heterosexual man | 906.32 | 1,214.51 | 1 | 5,768 | 338 |
| Ego is MSM | 657.79 | 765.25 | 1 | 5,435 | 360 |
| Ego lives in WEST | 541.92 | 691.17 | 2 | 5,244 | 272 |
| Ego lives in CENTRAL | 690.46 | 873.99 | 1 | 5,364 | 333.50 |
| Ego lives in EAST-CENTRAL | 739.01 | 1,061.46 | 1 | 5,561 | 312 |
| Ego lives in EAST | 668.27 | 920.58 | 3 | 5,164 | 273 |
| Ego lives in HAVANA | 715.67 | 812.44 | 1 | 5,768 | 416 |
| Ego is under 35 | 710.21 | 852.69 | 1 | 5,768 | 367 |
| Ego is over 35 | 503.54 | 682.54 | 1 | 4,895 | 251 |

Table 13: *Time in days between the detection of egos and alters for all the edges.*

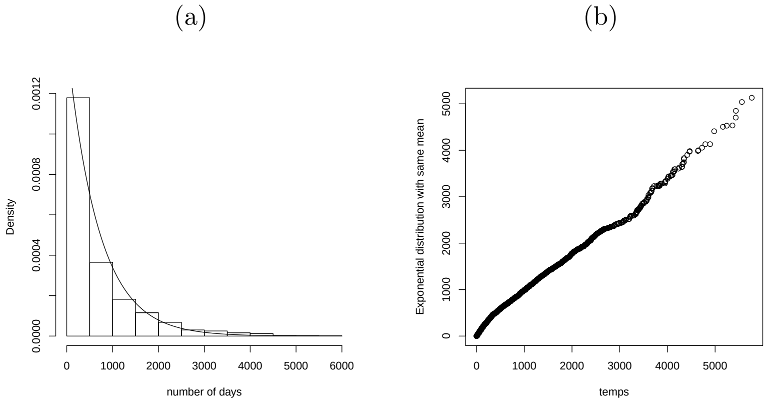


Figure 5: *(a) Histogramm of the time between the detections of Ego and Alter (in days). We added the density of the exponential distribution with same expectation. (b) Quantile-quantile plot of the time between detections of Ego and Alter with respect to the exponential distribution of same expectation.*

| Variable | Mean | Standard deviation | Minimum | Maximum | Median |
|---|---|---|---|---|---|
| Whole population | 665.68 | 818.56 | 1 | 5,768 | 336 |
| Ego is CONTA | 651.41 | 796.48 | 1 | 5,435 | 329 |
| Ego is CAPTA | 394.58 | 473.85 | 1 | 3,683 | 235 |
| Ego is RANDOM | 720.81 | 867.56 | 1 | 5,768 | 381 |
| Ego is woman | 654.41 | 854.12 | 1 | 4,795 | 293 |
| Ego is heterosexual man | 894.18 | 1,186.08 | 1 | 5,768 | 339 |
| Ego is MSM | 647.49 | 764.13 | 1 | 5,435 | 52 |
| Ego lives in WEST | 519.72 | 683.74 | 1 | 5,244 | 238 |
| Ego lives in CENTRAL | 646.53 | 809.41 | 1 | 4,795 | 325.50 |
| Ego lives in EAST-CENTRAL | 682.55 | 967.68 | 1 | 4,980 | 312 |
| Ego lives in EAST | 671.93 | 986.89 | 3 | 5,164 | 241 |
| Ego lives in HAVANA | 701.78 | 806.34 | 1 | 5,768 | 401 |
| Ego is under 35 | 687.76 | 834.39 | 1 | 5,768 | 350 |
| Ego is over 35 | 499.47 | 834.39 | 1 | 4,895 | 249 |

Table 14: *Time in days between the detection of egos and alters in the detection graph.*

# 4 Infection tree

Some light on the mechanisms of infection can be seen from the study of the infection tree. First and as expected, it appears in Table 15 that the infection propagates from the heterosexual men to the MSM through women. Cases of women infection by MSM is twice as much as the cases of infection by heterosexual men. In return, infected women infect heterosexual men and MSM in similar proportions: 39.56% and 53.58%. There is an important MSM core in the epidemic. 70% of the latter are infected by other MSM, 1,202 edges (52.56%) link two MSM, 667 edges (29.16%) link MSM and women and 375 edges (16.40%) links women and heterosexual men. We also see that there is an asymmetry: among infectious edges involving women, the latter are more often alters than egos (66.13% of the edges shared with heterosexual men and 74.21% of the edges shared with MSM).

Individuals detected by contact-tracing have been infected by 56.68% by individual who have been found by random detection, and by 43.32% by individuals detected by non-random methods, i.e. contact-tracing and captation (see Table 16). We compare the distribution of detection ways among individuals infected by egos found by contact-tracing or random detection. A $\chi^2$-test accepts with a p-value 75.97% that these distributions are the same. If we gather the individuals found by non-random methods, the $\chi^2$-test still accepts the equality of the distributions, but with a much lower p-value of 9.18%. Hence, that an individual is detected by non-random detection methods does not imply that we will have a lower chance of detecting the persons he/she has infected by contact-tracing or captation.

The study of geographic locations in the infection tree shows that infections mostly occur inside a same area. Only La Havana has relatively important connexions with the other regions. The frequencies of these connections have similar amplitudes (between 40 and 50 cases, if we consider edges with egos or alters in La Havana). Dealing with age-structure, 58.84% of the edges are between individuals in the age-class $[20, 40)$.

| | Alter is a woman | Alter is a heterosexual man | Alter is an MSM | Total |
|---|---|---|---|---|
| Ego is a Woman | 22 (6.85%, 2.88%) | 127 (39.56%, 90.71%) | 172 (53.58%, 12.95%) | 321 (*14.04%*) |
| Ego is a Heterosexual man | 248 (95.75%,32.42%) | 3 (1.16%,2.14%) | 8 (3.09%,0.60%) | 259 (*11.32%*) |
| Ego is a MSM | 495 (29.00%,64.71%) | 10 (0.59%,7.14%) | 1,202 (86.98%,70.42%) | 1,707 (*74.64%*) |
| Total | 765 (*33.45%*) | 140 (*6.12%*) | 1,382 (*60.43%*) | |

Table 15: *Sexual orientation of egos and alters for the edges in the infection tree. Frequency is given together with the row and column proportions between brackets. The diagonal of the contingency table represents 53,65% of the whole edges. The assortative mixing coefficient is* $r = 0.98957$.

| | Alter is CONTA | Alter is CAPTA | Alter is RANDOM | Total |
|---|---|---|---|---|
| Ego is CONTA | 410 (55.41%,32.59%) | 67 (9.05%, 31.46%) | 263 (35.54%,32.23%) | 740 (*32.36%*) |
| Ego is CAPTA | 135 (51.92%,10.73%) | 41 (15.77%,19.25%) | 84 (32.31%,10.29%) | 260(*11.37%*) |
| Ego is RANDOM | 713 (55.40%,56.68%) | 105 (8.16%,49.30%) | 469 (36.44%,57.48%) | 1,287 (*56.27%*) |
| Total | 1,258 (*55.01%*) | 213 (*9.31%*) | 816 (*35.68%*) | |

Table 16: *Type of detection of egos and alters for the edges in the infection tree. The diagonal of the contingency table represents 40.23% of the whole edges. The assortative mixing coefficient is* $r = 0.9899$.

| Ego is in | Alter is in WEST | Alter is in CENTRAL | Alter is in EAST-CENTRAL | Alter is in EAST | Alter is in HAVANA | Total |
|---|---|---|---|---|---|---|
| WEST | 204 | 8 | 2 | 0 | 23 | 237 |
| CENTRAL | 5 | 433 | 8 | 4 | 32 | 482 |
| EAST-CENTRAL | 1 | 3 | 76 | 5 | 13 | 98 |
| EAST | 5 | 2 | 6 | 266 | 21 | 300 |
| LA HAVANA | 25 | 22 | 23 | 38 | 1,062 | 1,170 |
| Total | 240 | 468 | 115 | 313 | 1,151 | |

Table 17: *Geographic location of egos and alters for the edges in the infection tree. The diagonal of the contingency table represents 89.24% of the whole edges. The assortative mixing coefficient is* $r = 0.9734$.

| | Alter is in $[10, 20)$ | Alter is in $[20, 30)$ | Alter is in $[30, 40)$ | Alter is in $[40, 50)$ | Alter is in $[50, 90)$ | Total |
|---|---|---|---|---|---|---|
| Ego is in $[10, 20)$ | 52 | 139 | 62 | 21 | 18 | 292 |
| Ego is in $[20, 30)$ | 129 | 505 | 349 | 89 | 41 | 1,113 |
| Ego is in $[30, 40)$ | 67 | 289 | 198 | 64 | 16 | 634 |
| Ego is in $[40, 50)$ | 12 | 73 | 53 | 18 | 7 | 163 |
| Ego is in $[50, 90)$ | 10 | 31 | 29 | 6 | 1 | 77 |
| Total | 270 | 1,037 | 691 | 198 | 83 | |

Table 18: *Age classes of egos and alters for the edges in the infection tree. The diagonal of the contingency table represents 33.96% of the whole edges. The assortative mixing coefficient is* $r = 0.9900$.

# 5 Degree distribution

The number $k(x)$ of edges connected to a given vertex $x$ is called its degree. The degree of an individual detected as HIV positive between 1986 and 2006 is stored in the variable 'ncontact' and corresponds to the number of sexual contacts in the two years preceding detection. Among the declared contacts, 'ncontest' provides the number of tested contacts, some of them having refused to take the HIV test or having not been found by the heath system. The number of seropositive contacts found is 'ncontpos' (see Table 19). Finally, there is also the observed degree, which

is the actual degree observed on the graph. The contact tested positive are in the database, but links that where not declared can be recovered by founding hidden partners afterwards, implying that the observed degree is larger than 'ncontpos'.

| | Mean | Std. dev. | Min | Max | Median |
|---|---|---|---|---|---|
| ncontact | 5.60 | 5.57 | 0 | 82 | 4 |
| ncontest | 4.31 | 4.84 | 0 | 74 | 3 |
| ncontpos | 0.95 | 1.29 | 0 | 19 | 1 |
| observed deg. in the graph | 1.51 | 1.82 | 0 | 21 | 1 |

Table 19: *Summary statistics for the declared degree, the number of tested contacts and the number of positive contacts for the whole population. The observed number of contacts in the graph is also given.*

## 5.1 Covariate description

Among the 5,389 individuals appearing in the database, 483 declared no sexual partners during the two years before detection. In Table 20, we give the degree distribution conditionally to various covariates. According to the result of one-way ANOVAs, that sexual orientation, way of detection, age at detection or geographic location do not impact the observed degree distribution, although some differences can be seen on the figures.

| Number of sexual partners | Mean | Std. dev. | Min | Max | Median |
|---|---|---|---|---|---|
| Whole population | 5.60 | 5.57 | 0 | 82 | 4 |
| WEST | 7.28 | 6.75 | 0 | 57 | 6 |
| CENTRAL | 7.47 | 7.02 | 0 | 58 | 6 |
| EAST-CENTRAL | 6.45 | 6.15 | 0 | 57 | 5 |
| EAST | 6.09 | 5.42 | 0 | 52 | 5 |
| HAVANA | 4.65 | 4.60 | 0 | 82 | 4 |
| Women | 5.54 | 5.08 | 0 | 39 | 4 |
| Heterosexual men | 4.25 | 4.18 | 0 | 30 | 3 |
| MSM | 5.82 | 5.86 | 0 | 82 | 5 |
| CONTA | 6.16 | 5.43 | 0 | 54 | 5 |
| CAPTA | 5.45 | 5.11 | 0 | 62 | 5 |
| RANDOM | 5.36 | 5.73 | 0 | 82 | 4 |
| Age $\in [10, 20)$ | 5.60 | 5.32 | 0 | 54 | 4 |
| Age $\in [20, 30)$ | 5.69 | 5.78 | 0 | 82 | 4 |
| Age $\in [30, 40)$ | 5.49 | 5.45 | 0 | 57 | 4 |
| Age $\in [40, 50)$ | 5.42 | 5.28 | 0 | 46 | 4 |
| Age $\in [50, 90)$ | 5.87 | 5.40 | 0 | 42 | 5 |

Table 20: *Number of declared contact 'ncontact'.*

Degree distributions are plotted in Fig. 6. All these distributions are highly *right-skewed* (i.e. with a long right-tail) and can be seen at a glance to exhibit a clear power-law behavior.

## 5.2 Calibration of power-law distributions

Based on the variable 'ncontact', we propose to fit a power-law exponent and use for this two methods which are described in Section 2.1 of the article.

### 5.2.1 Minization Küllback-Leibler divergence

When minimizing over $\alpha > 1$, the Küllback-Leibler divergence $\mathcal{K}_{k_0}(p, \alpha)$ that compares the observed distribution of '*ncontact*' to the power-law distribution with exponent $\alpha$ based on the values larger than $k_0$ for the degree, we obtain an estimator $\widehat{\alpha}_{k_0}$. We plot the graph of the mapping $k_0 \mapsto \mathcal{K}_{k_0}(p, \widehat{\alpha}_{k_0})$ (Fig. 7, left column), as well as that of the mapping $k_0 \geq 1 \mapsto \widehat{\alpha}_{k_0}$ (middle column).

The resulting estimates are $(k_0,\ \alpha) = (7,\ 3.06)$ for the pooled population, $(7,\ 3.02)$ for MSM, $(6,\ 2.71)$ for women and $(7,\ 3.36)$ for heterosexual men. We observe a non negligible fluctuation in the tail exponent, women corresponding to the heaviest tail, followed by MSM and heterosexual men (the smaller the tail exponent $\alpha$, the

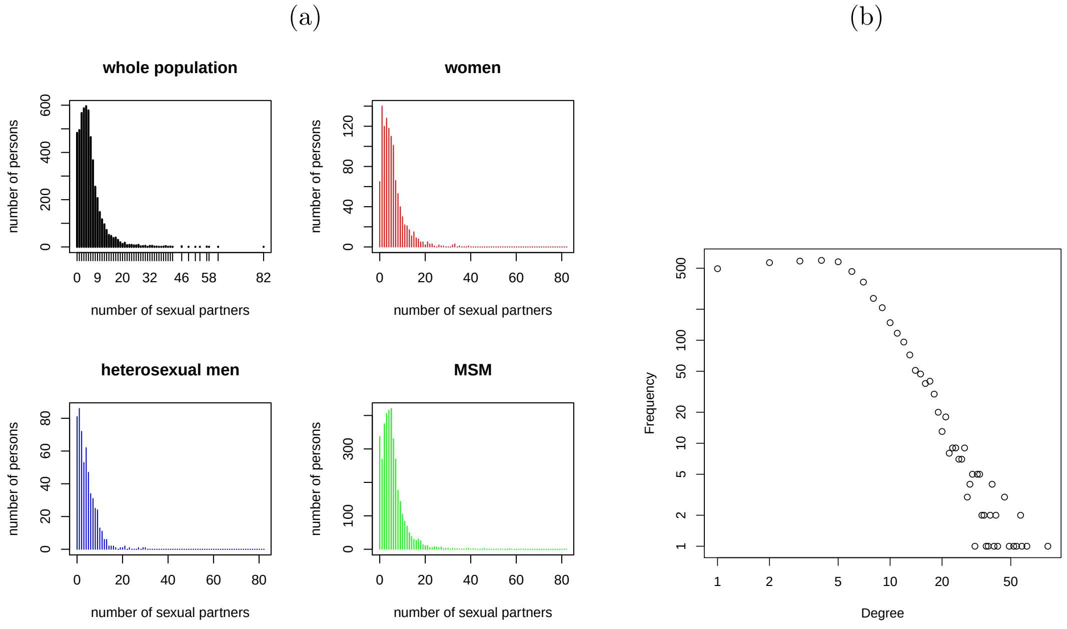


Figure 6: *(a) Degree distribution ('ncontact') for the population of individuals detected as HIV positive between 1986 and 2006, by sexual orientation. (b) Log-plot of the degree distribution for the whole population.*

| | $k_0$ | $\alpha$ |
|---|---|---|
| Whole population | 7 | 3.06 |
| Women | 6 | 2.71 |
| Heterosexual men | 7 | 3.36 |
| MSM | 7 | 3.02 |
| WEST | 6 | 2.49 |
| CENTRAL | 5 | 2.28 |
| EAST-CENTRAL | 7 | 2.80 |
| EAST | 6 | 2.80 |
| HAVANA | 6 | 3.28 |
| Age $[10, 20)$ | 6 | 2.84 |
| Age $[20, 30)$ | 6 | 2.85 |
| Age $[30, 40)$ | 6 | 2.88 |
| Age $[40, 50)$ | 5 | 2.66 |
| Age $[50, 90)$ | 5 | 2.62 |

Table 21: *Estimator of $\widehat{k}_0$ and $\widehat{\alpha}_{k_0}$ obtained when stratifying the population by sexual orientation, geographical location or age class. In the last part of the table, the age classes correspond to the ages at detection, and we retain only the classes with more than 25 individuals (see Table 4).*

heavier the distribution tail). More significantly, tail exponent estimates are higher for egos living in La Havana, see Table 21. For age classes, the estimated exponents are in constrat very similar.

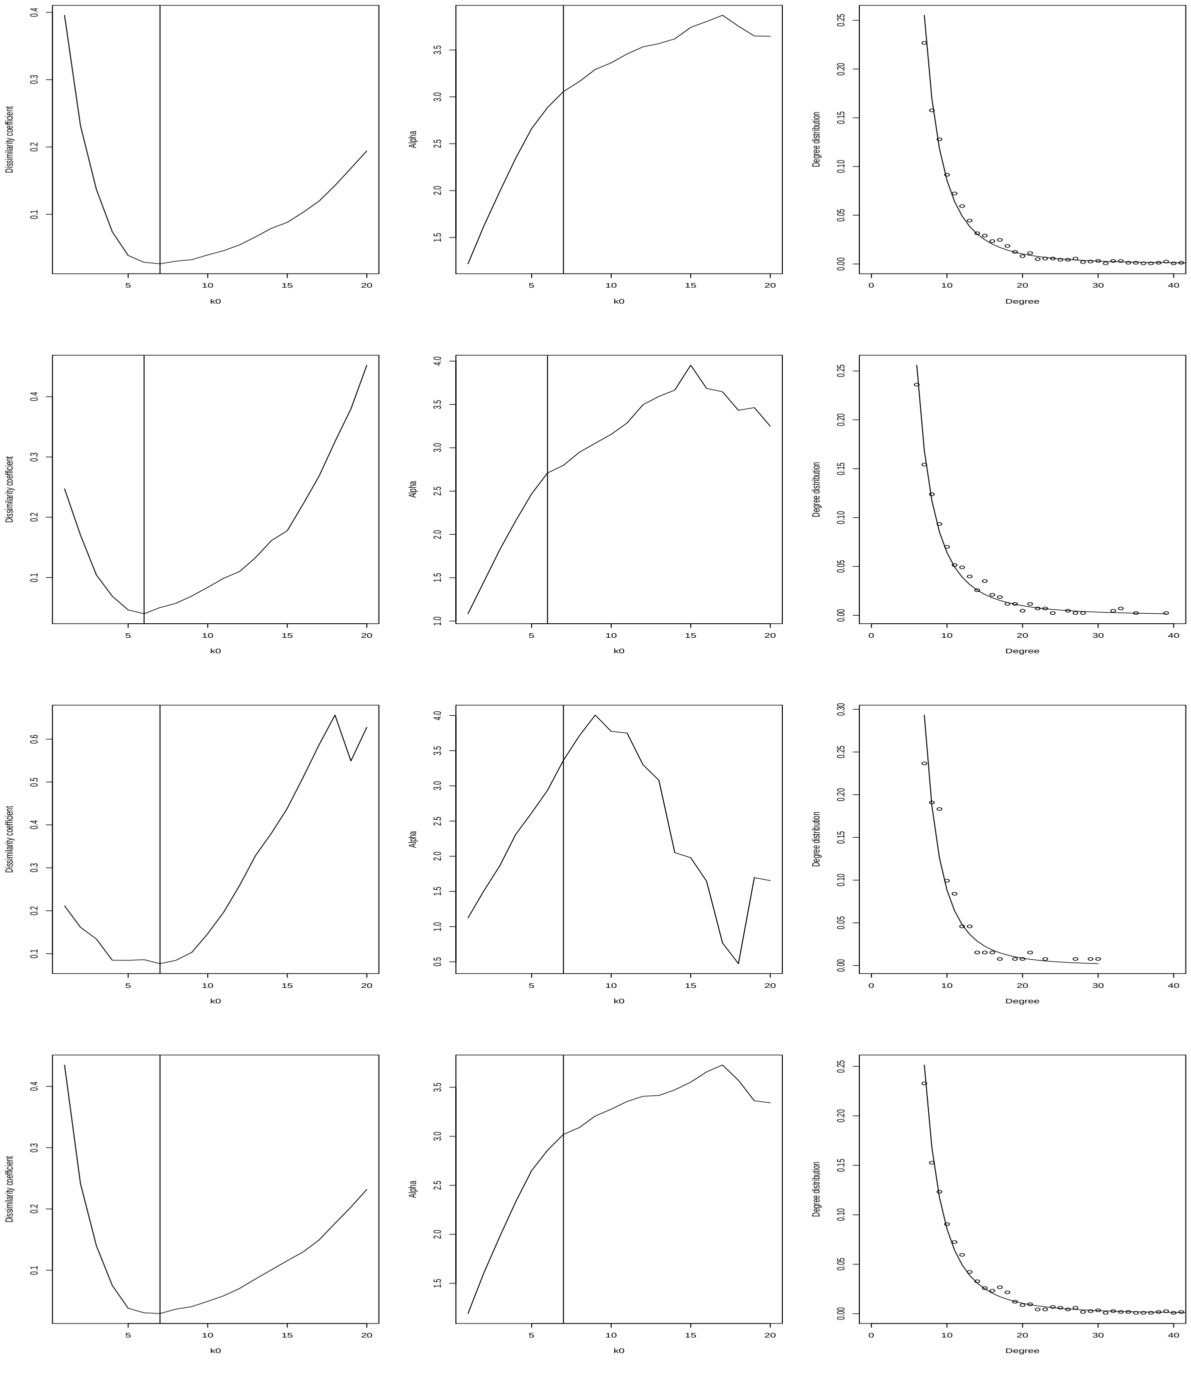


Figure 7: *(a) Dissimilarity measure* $\mathcal{K}_{k_0}(p, \widehat{\alpha}_{k_0})$ *as a function of* $k_0$*. The vertical lines indicate the value of the threshold yielding minimum discrepancy. (b) Estimator of* $\widehat{\alpha}_{k_0}$ *as a function of* $k_0$*. (c) Data and estimated power law. First line: Pooled population. Second line: women. Third line: heterosexual men. Fourth line: MSM.*

### 5.2.2 Hill estimator of the power

A *Hill estimator* $\widetilde{\alpha}_m$ of the parameter $\alpha$ is also considered, by retaining the $m$ highest observations. Reassuringly, we found that both estimation methods yield similar results.

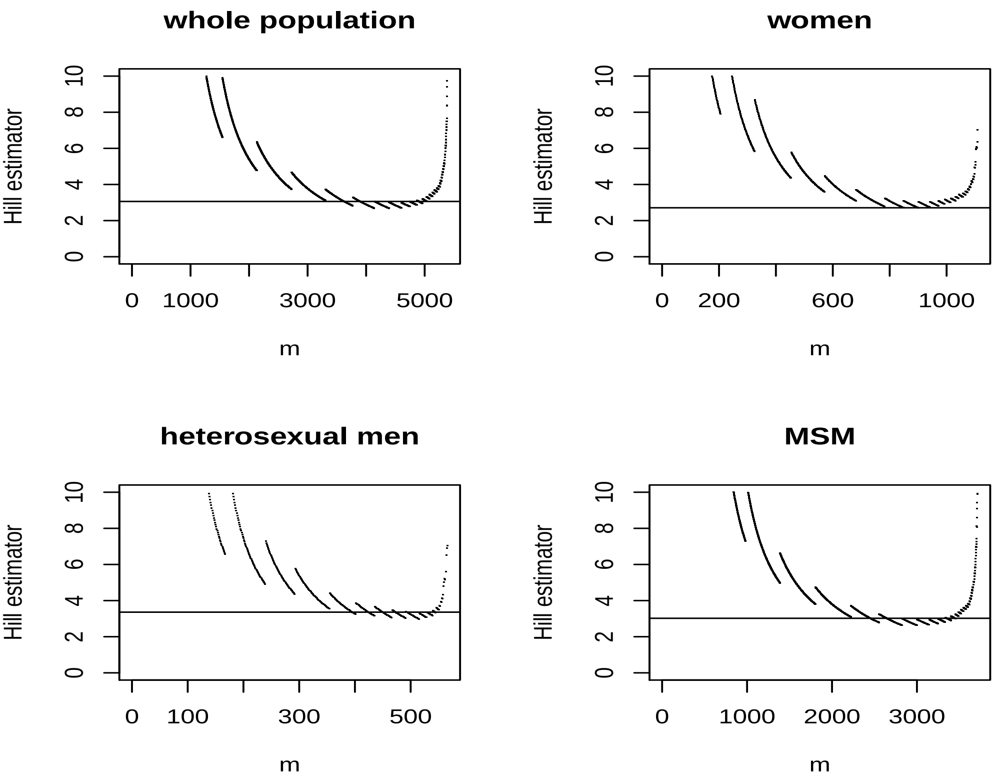


Figure 8: *Graph of* $(m, \widetilde{\alpha}_m)$ *for* $m \in \{1, \ldots, n\}$. *This graph allows to choose the Hill estimator. The horizontal line* $y = \widehat{\alpha}_{k_0}$ *permits to visualize the estimator* $\widehat{\alpha}_{k_0}$ *and compare it with the Hill estimator.*

| | $\alpha$ | $m$ |
|---|---|---|
| Whole population | 2.68 | 4,393 |
| Women | 2.71 | 901 |
| Heterosexual men | 2.98 | 515 |
| MSM | 2.63 | 3,001 |
| WEST | 2.74 | 398 |
| CENTRAL | 2.58 | 632 |
| EAST-CENTRAL | 2.87 | 276 |
| EAST 4 | 2.60 | 554 |
| HAVANA | 2.54 | 2,628 |
| Age $[10, 20)$ | 2.64 | 447 |
| Age $[20, 30)$ | 2.65 | 2,083 |
| Age $[30, 40)$ | 2.61 | 1,366 |
| Age $[40, 50)$ | 2.53 | 435 |
| Age $[50, 90)$ | 2.55 | 164 |

Table 22: *Hill estimators obtained when stratifying the population respectively by sexual orientation, geographical location and age class. It can be seen that the estimated exponents* $\widetilde{\alpha}_m$ *are often smaller than the estimators* $\widehat{\alpha}_{k_0}$.

## 5.3 Prediction of the appearance of the giant component

The giant component is studied separately in Section 7. Under the assumption that the network of sexual contacts is distributed as a configuration model, criteria exist for the possible emergence of a giant component (see [9, Eq. (28)] or [8]). Namely, a giant component in a configuration model graph with degree distribution $(p_k : k \in \mathbb{N})$ exists if

and only if $\sum_{k\geq 2} k(k-2)p_k > 0$. For the empirical degree distribution in the data (i.e. the observed degree of the individuals in the graph), the quantity above is positive, it is equal to 2.58. The occurrence of a giant component in the graph of sexual contacts involving individuals who have been diagnosed HIV positive before 2006 is thus no surprise.

The percolation threshold can also be analyzed using similar tools. In particular, the minimum edge based infection probability can be computed based on the declarative degree distribution for the whole population, and is equal to 9.87%. For the MSM sub-population, we obtain 9.33%. Those values are somewhat compatible with the transmission probabilities (see `http://en.wikipedia.org/wiki/AIDS`). Indeed the highest risk of transmission per intercourse is estimated as 5/1000. In order to reach the probabilities calculated above, approximately 19.5 unprotected intercourses should take place between each pair of connected partners, if the assumption of a configuration model graph is satisfied.

Would the graph be a configuration model graph, the coverage of the giant component, as predicted by [9] is of the order of 90% which is much higher than what is observed on our data. It should be noted that in [9], the coverage depends on the transmission probability for 1 intercourse (see Figure 9). The threshold value of the latter depend on the degree distribution. Using the actual observed graph which nodes have clearly lower actual degree that the declarative one, we obtain that a giant component is expected with a coverage of 56.6% of the graph. The subgraph of MSM is also expected to contain a giant component which should cover 47.3% of the nodes.

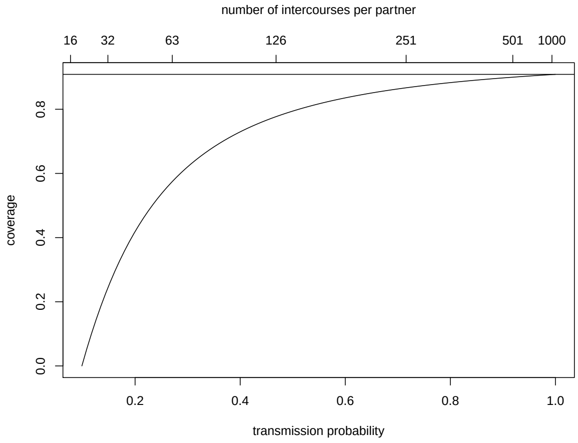


Figure 9: *Coverage as a fonction of the transmission probability/number of intercourse per partner, as estimated from the giant component.*

## 5.4 Isolated individuals

There are 1,627 isolated individuals. For these individuals, the covariate distributions do not reflect the ones of the whole population, as confirm $\chi^2$-tests. There are much more heterosexual men (16.59%) and less women (12.29%) than in the whole population. MSM are of the order of 70% in both samples. In the respect of methods of detection, only 3.20% of the isolated individuals have been detected by contact-tracing, 22.13% have been detected by captation and 74.68% by random methods. 64.23% of the isolated individuals live in La Havana. The other regions gather between 7% and 11% of these individuals.
For the isolated individuals, the mean number of contacts is 3.88 and the median is 3 (in comparison, the means are 5.60 and 6.92 for the whole population and giant component respectively). The main reason why these individuals are isolated is that they have few positive contacts: 99.88% have no positive contacts although 22.06% only declare no contact at all and 28.95% have no contact found (see Table 23). For comparison, the percentages of individuals who declare no contact in the whole population and giant component respectively are 8.96% and 2.80% (the latter being alters of other individuals of the giant component) and the percentages of individual bringing no new positive detection are 44.13% and 16.39% respectively.

| | Mean | Std. dev. | Min | Max | Median |
|---|---|---|---|---|---|
| ncontact | 3.89 | 4.43 | 0 | 57 | 3 |
| ncontest | 2.67 | 3.77 | 0 | 55 | 2 |
| ncontpos | 0.001 | 0.035 | 0 | 1 | 0 |

Table 23: *Summary statistics for the declared degree, the number of tested contacts and the number of positive contacts among the isolated individuals.*

Isolated couples are composed of many couples man-woman with a sur-representation of women compared with the whole information of the database.

# 6 Statistical summary of the graph

A wide variety of statistics are computed to summarize the properties of the network of large size.
Before analyzing in detail the giant component of the graph, we describe the density of the network. As we will see, the network density is globally low. However, it is very heterogeneous. As will be confirmed below by the analysis of the community structure of the giant component, although the connectivity properties of the network seem fragile at first glance, density may be locally very high.

## 6.1 Assortative mixing coefficients

| | Alter is a woman | Alter is a heterosexual man | Alter is an MSM | Total |
|---|---|---|---|---|
| Ego is a Woman | 77 (11.99%,6.64%) | 157 (24.45%,84.41%) | 408 (63.55%,14.96%) | 642 (*15.76%*) |
| Ego is a Heterosexual man | 282 (92.16%,24.33%) | 4 (1.31%,2.15%) | 20 (6.54%,0.73%) | 306 (*7.51%*) |
| Ego is a MSM | 800 (25.60%,69.03%) | 25 (0.80%,13.44%) | 2,300 (73.60%,84.31%) | 3,125 (*76.72%*) |
| Total | 1,159 (*28.46%*) | 186 (*4.57%*) | 2728 (*66.98%*) | |

Table 24: *Sexual orientation of egos and alters for the edges in the whole graph. Frequencies are given together with row and column proportions between brackets. The diagonal of the contingency table represents 58,46% of the whole edges. The assortative mixing coefficient is* $r = 0.0512$. *The independence between the sexual orientation of egos and alters is rejected by a* $\chi^2$*-test with a p-value smaller than* $2.2\,10^{-16}$. *In theory, there should be no sexual contact between two heterosexual men or between a heterosexual man and an MSM. The semantic of the database also exclude sexual contact between women. However, those events actually occur in the dataset.*

When considering the sexual orientation of egos and alters (Tables 24), we see that more than a half of the edges (56.47%) link two MSM. Links between MSM and women make 1,208 edges (29.66%) and there are 439 edges (10.78%) between women and heterosexual men. For the geographic location, as shown in Table 17, the vast majority of infections unsurprisingly occur inside the geographical regions considered: 2,041 (89.24%) of the 2,287 edges of the infection tree correspond to a pair of adjacent vertices in the same geographical location, and among those, 1,062 (46.43%) link two individuals belonging to La Havana and 433 (18.93%) link two individuals of Central. This results in a very high assortative mixing coefficient of $0.9734$.
When considering the joint distribution of age at detection, we see again a strong dependence. Not surprisingly, edges where alters and egos are between 20 and 40 make 58.84% of the edges in the infection tree. For the age-classes, we have an assortative mixing coefficient $r = 0.9899$, showing that as expected, egos and alters often have close ages.

## 6.2 Clustering properties

### 6.2.1 Clustering coefficients

In order to analyze the transitivity properties of a network, one can computes the *clustering coefficient* $C$. A network is said to be transitive when, given three vertices $A$, $B$ and $C$ such that $A$ is connected to $B$, who is itself connected to $C$, chosen at random, vertices $A$ and $C$ are also connected with large probability. We compute the clustering coefficient:

$$C = \frac{3 \times \mathcal{T}}{\mathbf{T}},$$

where $\mathcal{T}$ denotes the number of triangles within the network and $\mathbf{T}$ the number of connected triples of vertices, see [1]. Following in the footsteps of [11], a local version of this quantity can also be considered. For any vertex $x$ of the graph, the related local clustering coefficient is

$$C(x) = \frac{\mathcal{T}(x)}{\mathbf{T}(x)},$$

denoting by $\mathcal{T}(x)$ the number of triangles connected to $x$ and by $\mathbf{T}(x)$ the number of triples "centered at $x$", i.e. of the type $(y, x, z)$ where $y$ and $z$ are two distinct vertices of the graph, distinct from $x$. As an alternative, one may then consider $\widetilde{C} = \frac{1}{n}\sum_{x\in\mathcal{V}} C(x)$ for measuring transitivity within the network.

|  | $\mathcal{T}$ | **T** | C |
|---|---|---|---|
| Whole population | 177 | 10,673 | $4.98\,10^{-2}$ |
| MSM community | 100 | 5,068 | $5.92\,10^{-2}$ |
| MSM and women | 167 | 9,689 | $5.17\,10^{-2}$ |

Table 25: *Clustering coefficient* C*, together with the number of triangles* $\mathcal{T}$ *and the number of connected triples of vertices.*

The clustering coefficients and number of triangles are computed in Table 25. The clustering coefficients C are very small and show that there are few triads in the graph. The majority of the nodes have at most one contact in the database and therefore for 3509 vertices (out of 5389), no local clustering coefficient can be calculated. The graph shows a very low transitivity, which is also reflected by the computation of the local clustering coefficients of Table 26 for the giant component.

| Population | min | max | median | mean | std dev |
|---|---|---|---|---|---|
| Whole population | 0 | 1 | 0 | 0.0215 | 0.1210 |
|  | *0* | *1* | *0* | *0.1475* | *0.3190* |
| Giant component | 0 | 1 | 0 | 0.0406 | 0.1597 |
|  | *0* | *1* | *0* | *0.2057* | *0.3417* |
| Women | 0 | 1 | 0 | 0.0303 | 0.1344 |
|  | *0* | *1* | *0.4167* | *0.5209* | *0.3665* |
| Heterosexual men | 0 | 1 | 0 | 0.0258 | 0.1409 |
|  | *0* | *1* | *0.4000* | *0.4411* | *0.4172* |
| MSM | 0 | 1 | 0 | 0.0442 | 0.1666 |
|  | *0* | *1* | *0* | *0.1089* | *0.2647* |
| WEST | 0 | 1 | 0 | 0.0733 | 0.1906 |
|  | *0* | *1* | *0.2135* | *0.3392* | *0.3816* |
| CENTRAL | 0 | 1 | 0 | 0.0406 | 0.1511 |
|  | *0* | *1* | *0.1667* | *0.2972* | *0.3615* |
| EAST-CENTRAL | 0 | 0.1 | 0 | 0.0015 | 0.0124 |
|  | *0* | *1* | *0* | *0.1494* | *0.3295* |
| EAST | 0 | 1 | 0 | 0.0331 | 0.1506 |
|  | *0* | *1* | *0* | *0.2015* | *0.3544* |
| HAVANA | 0 | 1 | 0 | 0.0441 | 0.1666 |
|  | *0* | *1* | *0* | *0.1471* | *0.3079* |
| Age in $[10, 20)$ | 0 | 1 | 0 | 0.0500 | 0.1724 |
|  | *0* | *1* | *0* | *0.2325* | *0.3436* |
| Age in $[20, 30)$ | 0 | 1 | 0 | 0.0393 | 0.1586 |
|  | *0* | *1* | *0* | *0.2088* | *0.3415* |
| Age in $[30, 40)$ | 0 | 1 | 0 | 0.0436 | 0.1643 |
|  | *0* | *1* | *0* | *0.2006* | *0.3422* |
| Age in $[40, 50)$ | 0 | 1 | 0 | 0.0262 | 0.1277 |
|  | *0* | *1* | *0* | *0.1826* | *0.3437* |
| Age in $[50, 90)$ | 0 | 1 | 0 | 0.0382 | 0.1659 |
|  | *0* | *1* | *0* | *0.1783* | *0.3286* |

Table 26: *Main features of the distribution of the local clustering coefficient* $C(x)$ *depending on the population considered. Apart from the first row (whole population), all statistics are computed on the restriction to the giant component. In italic script, we give the statistics for the local clustering coefficient with the correction inspired from bipartite graphs: i.e. adding edges between heterosexual men or women having a common neighbor in the original sexual contact graph.*

Moreover, because of the semantics of the edges, only some specific type of cliques are expected to arise in the Cuban dataset. In this respect, we recall that a *clique* $\mathcal{C}$ is a subset of vertices, all adjacent, and it is said *maximal* if there is no clique into which it is strictly included. The full graph contains 187 possibly overlapping cliques of at least 3 members. The vast majority (177 among 187) of the cliques contain only three persons. We remove non maximal size 3 cliques which leads to a total of number of maximal cliques of 150 from which 10 have four members. Most of the cliques belong to the largest connected component (this is the case for all four members cliques). There are nevertheless 10 three member cliques in other connected components.
Among the cliques with four members, 5 are constituted only of MSM, and 3 are made of 3 men and 1 woman.

### 6.2.2 Global path length

The diameter of the graph is 36 when orientation is taken into account and 26 without orientation. As the graph is not connected, the diameter is obtained as the largest diameter of the connected components. In the present case it is the diameter of the largest connected component.

Average geodesic path lengths can also be computed. Since, the graph is highly disconnected, with 1,627 isolated nodes and 308 pairs of isolated nodes, the average geodesic path length is only meaningful in the connected components. It turns out that most of the connectivity is concentrated in the largest component (3,168 edges out of 4,073), where the averages geodesic path lengths are 12.23 with orientation and 10.24 without. Those values are rather high compared to values given in Newman's survey but remain well below the number of vertices and compatible with the logarithmic scaling associated to the small world effect.

We calculated average geodesics and diameters on the largest connected component, considered as an undirected graph, taking additionally into account the covariates (Tables 27). The diameters are always of the order of 25 nodes. Geodesics have also similar lengths, but the shortest geodesics link heterosexual men and women or between individuals detected by contact-tracing, which was expected.

| | MSM | heterosexual man | woman |
|---|---|---|---|
| MSM | 10.30, *25.00* | 10.83, *26.00* | 10.24, *25.00* |
| heterosexual man | 10.83, *26.00* | 9.87, *25.00* | 9.30, *25.00* |
| woman | 10.24, *25.00* | 9.30, *25.00* | 8.76, *24.00* |

Table 27: *Average geodesic distances and diameters (in italic) in the giant component.*

| | CAPTA | CONTA | RANDOM |
|---|---|---|---|
| CAPTA | 10.85, *25.00* | 10.68, *25.00* | 10.76, *25.00* |
| CONTA | 10.68, *25.00* | 9.73, *26.00* | 10.13, *26.00* |
| RANDOM | 10.76, *25.00* | 10.13, *26.00* | 10.36, *25.00* |

Table 28: *Average geodesic distances and diameters (in italic) in the giant component.*

## 6.3 Network resilience, shortest-path centrality

In connection with the degree distribution analysis, one may investigate how the connectivity properties of the network evolve when removing various fractions of specific strata of the population. A vertex in a connected graph is called an articulation point, when removing it and all edges incident to it results in a non-connected graph. More generally, a network is said to exhibit resilience, when removal of certain vertices does not affect much its communication structure.

As proposed by [6], resilience with respect to a specific vertex can be measured by betweenness centrality, which is the number of geodesic paths between other vertices that run through it. In order to explore resilience with respect to a certain stratum (defined by the variable 'age at detection', 'sexual orientation' respectively), we draw at random fractions of vertices to remove and recompute statistics of interest (geodesic distances, degree distributions, size of the largest component...), the latter being averaged next over many replications of the random removal.

In this respect, we have determined the articulation points of the connected components of the graph. Because of this low density, the graph is expected to contain many articulation points. The computation indeed exhibits 1,157 nodes that are articulation points. We see that most of them are MSMs (74.24% for the whole graph and 78.05% for the giant component). The distribution of the sexual orientation among the articulation points is strongly different from the sexual orientation in the whole graph, as shown by a $\chi^2$-test with p-value 0.0001732. However, this is not the case inside the largest connected component, as reveals a $\chi^2$-test with p-value 0.2296. This might be explained by the fact that the largest connected component is already quite different from the general dataset in term of sexual orientation.

Several centrality measures can be used to detect interesting persons in the graph and also to measure the importance of some groups in term of connectivity. The degree of a node is possibly the simplest of such measure. In the Cuban dataset, we have two degrees: the declarative number of sexual contacts and the actual number of infected contacts. Other connectivity based measures can be used, such as the node betweenness centrality and the closeness centrality (centrality is interesting only in connected graphs). For those four measures, one can study the distribution of the node characteristics of the top persons, the consensus between the measures in term of node ranking, etc. For instance, the Figure 10 displays the sexual orientation of the persons ordered according to centrality measures. It

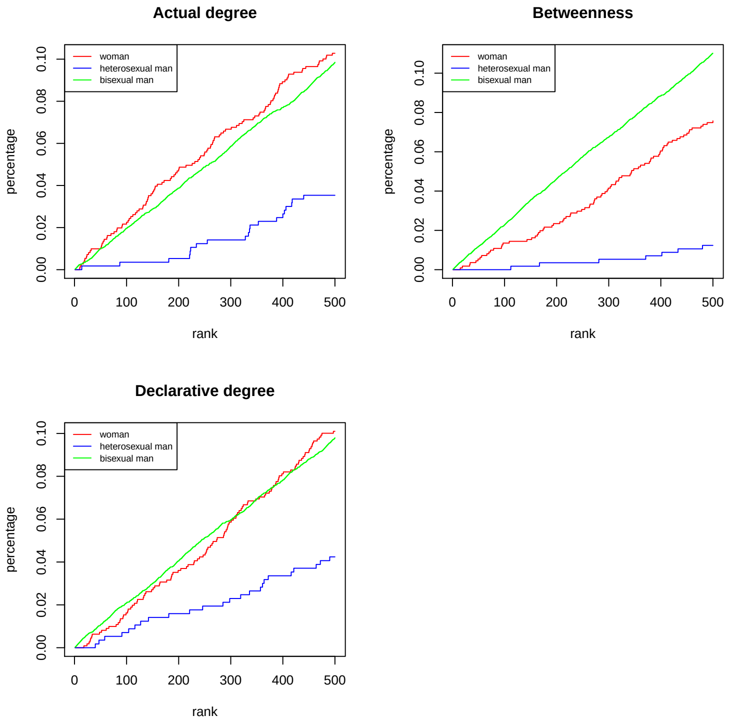


Figure 10: *Sexual orientation with respect to centrality measures, for the whole population. More precisely, each graph shows the percentage of the total women (for instance) included in the top* $n$ *nodes according to the chosen measure, for increasing values of* $n$*.*

appears clearly that the three measures strongly disagree on the ranking of the nodes. This is quite logical according to the definition of the measures. The declarative degree shows a smaller mean degree for heterosexual men and comparable degree distribution between women and MSM. This is reflected in the ranking. The actual degree gives lower ranks to heterosexual men who are connected only to women. MSM are expected to contribute most to the connectivity of the graph, especially bisexual men who act as contact points between women and homosexual men.

Similar studies can be carried for the largest connected component (see Fig. 11), including this time the closeness centrality measure (which is not adapted to non connected graphs).

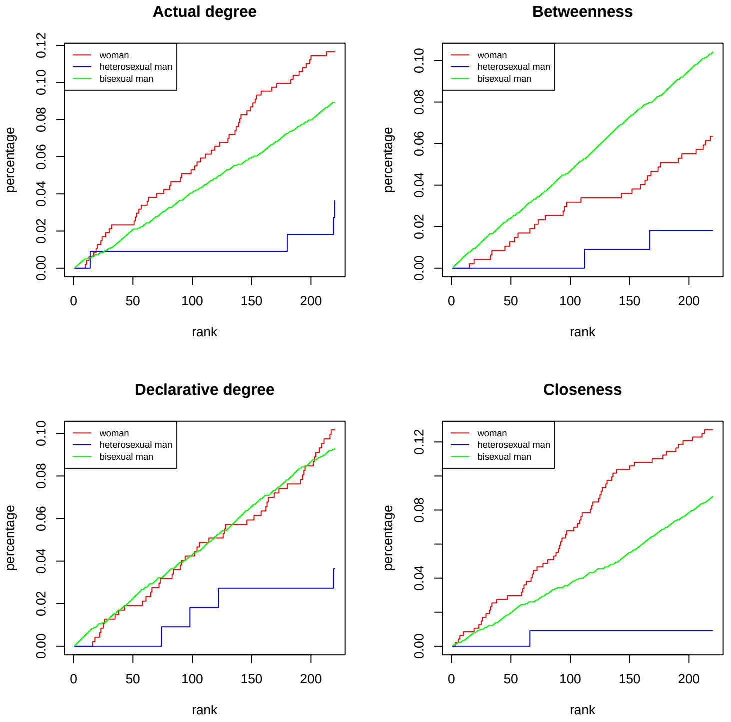


Figure 11: *Sexual orientation with respect to centrality measures, for individuals in the giant component.*

# 7 Study of the giant component

## 7.1 Covariate distribution

First, let us give the characteristics of the giant component in terms of sexual orientation and geographical location. A $\chi^2$ test for comparing the distribution of sexual orientation in the giant component with that of the whole population says that there is a significant difference in these two distributions: there are more MSMs in the giant component, which is composed by 19.87% of women, by 4.61% of heterosexual men and by 75.61% of MSMs. All the same, there is a significant difference between the mode of detection of these individuals, who are at 40.23% and 10.48% detected by contact-tracing and captation, *i.e.* non-random methods.

| | WEST | CENTRAL | EAST-CENTRAL | EAST | HAVANA |
|---|---|---|---|---|---|
| Frequency | 236 | 548 | 65 | 223 | 1,314 |
| Proportion | 9.89% | 22.97% | 2.72% | 9.35% | 55.07% |

Table 29: *Distribution by geographic location. A $\chi^2$-test tells that the geographical distributions for the whole population and for the giant component significantly differ.*

| | Mean | Std. dev. | Min | Max | Median |
|---|---|---|---|---|---|
| ncontact | 6.92 | 6.30 | 0 | 82 | 5 |
| ncontest | 5.54 | 5.44 | 0 | 74 | 4 |
| ncontpos | 1.65 | 1.55 | 0 | 19 | 1 |

Table 30: *Summary statistics for the declared degree, the number of tested contacts and the number of positive contacts for the individual of the giant component.*

## 7.2 Supplementary material for the clustering of the giant component

The giant component is analyzed in depth in the main document [4]. We provide here supplementary figures and graphs that complement the analysis. A film showing the growth of the clusters of the giant component is in supplementary materials: `animation.mp4`. In this film, the clusters appear and grow. The colors correspond to the growth rates: light colors indicate little variation in the cluster size while dark red correspond to expanding clusters.

Among the 37 clusters listed in Table 32, 22 exhibit a distribution for 'sexual orientation' that is significatively different from the one in the whole dataset. These clusters are referred to as "atypical clusters" that can themselves be separated into two classes, depending on whether the proportion of MSM is higher or less than the one in the giant component. The two groups are referred to as the "MSM clusters" and the "mixed clusters". The distributions of the 'sexual orientation' in the atypical clusters and in the other clusters are shown in Table 31.

| | absolute | relative |
|---|---|---|
| **MSM clusters** | | |
| MSM | 748 | 0.97 |
| Heterosexual men | 4 | 0.01 |
| Women | 22 | 0.03 |
| **Mixed clusters** | | |
| MSM | 452 | 0.55 |
| Heterosexual men | 70 | 0.08 |
| Women | 303 | 0.37 |
| **Other clusters** | | |
| MSM | 604 | 0.77 |
| Heterosexual men | 36 | 0.05 |
| Women | 147 | 0.19 |

Table 31: *Sexual orientation distribution in the groups of MSM, mixed and other clusters, both in absolute number of persons and in relative numbers*

| | MSM | Mixed | Other |
|---|---|---|---|
| MSM | 9.95 | 13.51 | 11.97 |
| Mixed | 13.51 | 7.28 | 9.92 |
| Other | 11.97 | 9.92 | 12.50 |

Table 32: *Mean geodesic distances between subgroups of the giant component*

| Cluster | Vertices | p-value | MSM | Heterosexual men | Women |
|---|---|---|---|---|---|
| | 2386 | | 0.756 | 0.046 | 0.198 |
| 14 | 66 | 0.0001 | 0.500 | 0.061 | 0.439 |
| 26 | 13 | 0.0001 | 0.000 | 0.462 | 0.538 |
| 27 | 141 | 0.0001 | 0.496 | 0.113 | 0.390 |
| 34 | 38 | 0.0001 | 0.158 | 0.211 | 0.632 |
| 5 | 94 | 0.0002 | 0.979 | 0.000 | 0.021 |
| 33 | 131 | 0.0003 | 0.588 | 0.053 | 0.359 |
| 6 | 66 | 0.0004 | 0.985 | 0.000 | 0.015 |
| 20 | 64 | 0.0004 | 0.984 | 0.000 | 0.016 |
| 7 | 63 | 0.0007 | 0.984 | 0.000 | 0.016 |
| 28 | 141 | 0.0007 | 0.617 | 0.050 | 0.333 |
| 21 | 65 | 0.0008 | 0.985 | 0.015 | 0.000 |
| 16 | 66 | 0.0013 | 0.970 | 0.000 | 0.030 |
| 23 | 63 | 0.0013 | 0.984 | 0.000 | 0.016 |
| 30 | 134 | 0.0014 | 0.612 | 0.082 | 0.306 |
| 32 | 75 | 0.0017 | 0.960 | 0.000 | 0.040 |
| 22 | 65 | 0.0019 | 0.954 | 0.015 | 0.031 |
| 4 | 10 | 0.0024 | 0.200 | 0.200 | 0.600 |
| 17 | 9 | 0.0103 | 0.333 | 0.000 | 0.667 |
| 19 | 45 | 0.0106 | 0.956 | 0.000 | 0.044 |
| 3 | 142 | 0.0122 | 0.648 | 0.063 | 0.289 |
| 2 | 41 | 0.0207 | 0.951 | 0.000 | 0.049 |
| 24 | 67 | 0.0237 | 0.896 | 0.030 | 0.075 |
| 10 | 54 | 0.0615 | 0.889 | 0.037 | 0.074 |
| 31 | 62 | 0.0656 | 0.645 | 0.097 | 0.258 |
| 13 | 34 | 0.0813 | 0.912 | 0.000 | 0.088 |
| 12 | 14 | 0.0829 | 0.571 | 0.000 | 0.429 |
| 36 | 54 | 0.1130 | 0.722 | 0.000 | 0.278 |
| 8 | 8 | 0.2949 | 1.000 | 0.000 | 0.000 |
| 18 | 72 | 0.3039 | 0.833 | 0.028 | 0.139 |
| 15 | 48 | 0.3958 | 0.812 | 0.062 | 0.125 |
| 29 | 18 | 0.4173 | 0.667 | 0.111 | 0.222 |
| 11 | 83 | 0.4439 | 0.711 | 0.072 | 0.217 |
| 0 | 33 | 0.7115 | 0.697 | 0.061 | 0.242 |
| 9 | 124 | 0.7597 | 0.774 | 0.032 | 0.194 |
| 35 | 115 | 0.7890 | 0.774 | 0.052 | 0.174 |
| 25 | 29 | 0.8287 | 0.724 | 0.034 | 0.241 |
| 1 | 39 | 0.8312 | 0.795 | 0.051 | 0.154 |

Table 33: Sexual orientation distribution among the 37 clusters, numbered from 0 to 36. Proportions are given in columns 4-6. The table orders the clusters via the p-value of a $\chi^2$-square test of adequation with the global sexual orientation distribution in the data conducted on each cluster. Those p-values show that numerous clusters have a sexual orientation distribution which is significantly different from the global distribution in the largest connected component.

## 7.3 The 37 clusters of the giant component

The 37 subgraphs obtained when clustering the giant component, numbered from 0 to 36, are finally represented.

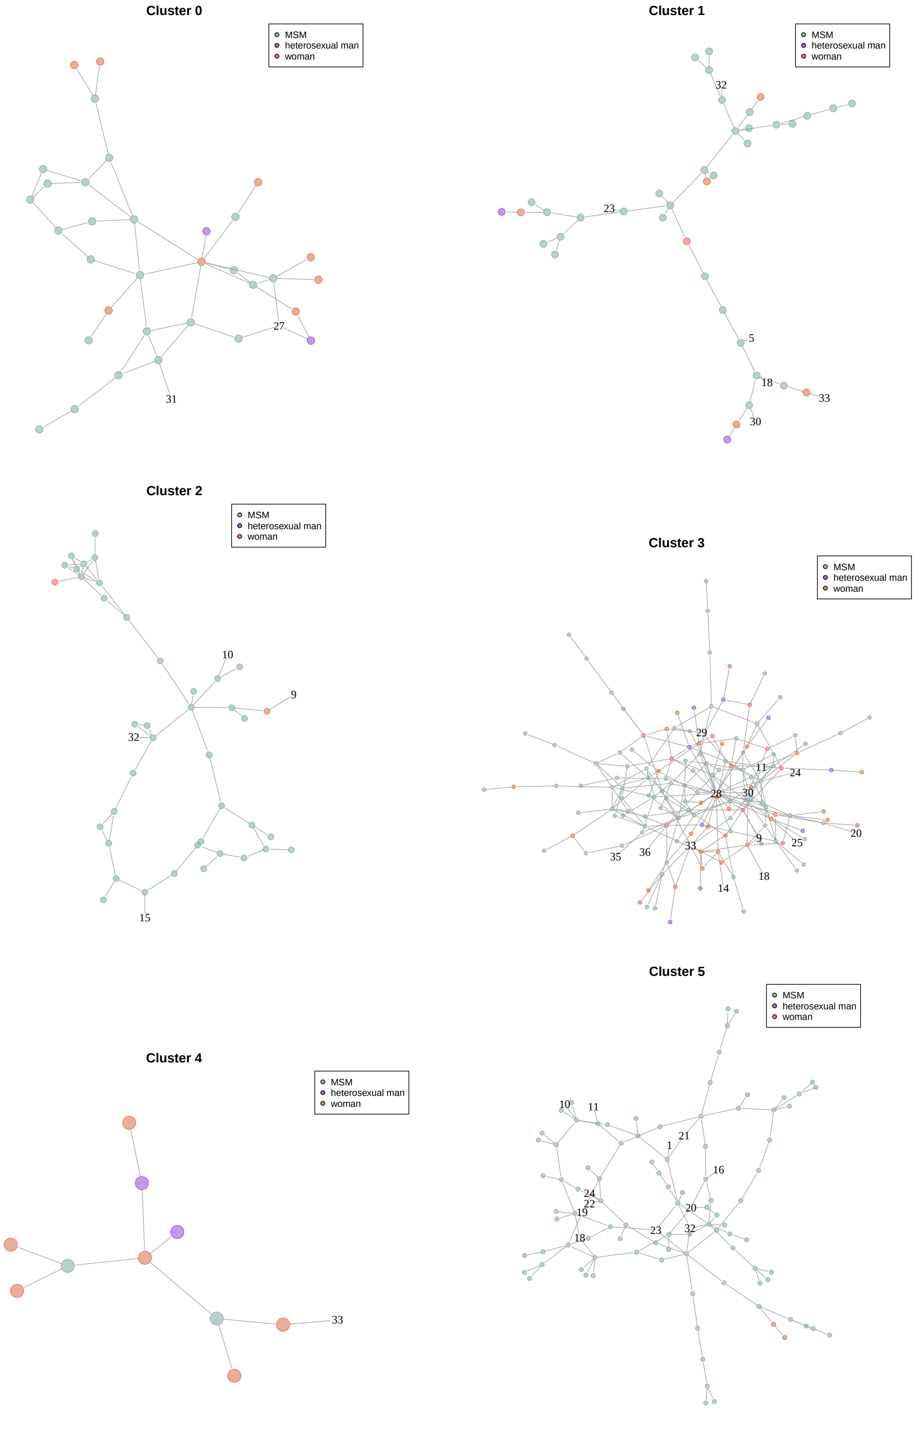


Figure 12: *Clusters from the largest connected components. Numbered nodes represent other clusters.*

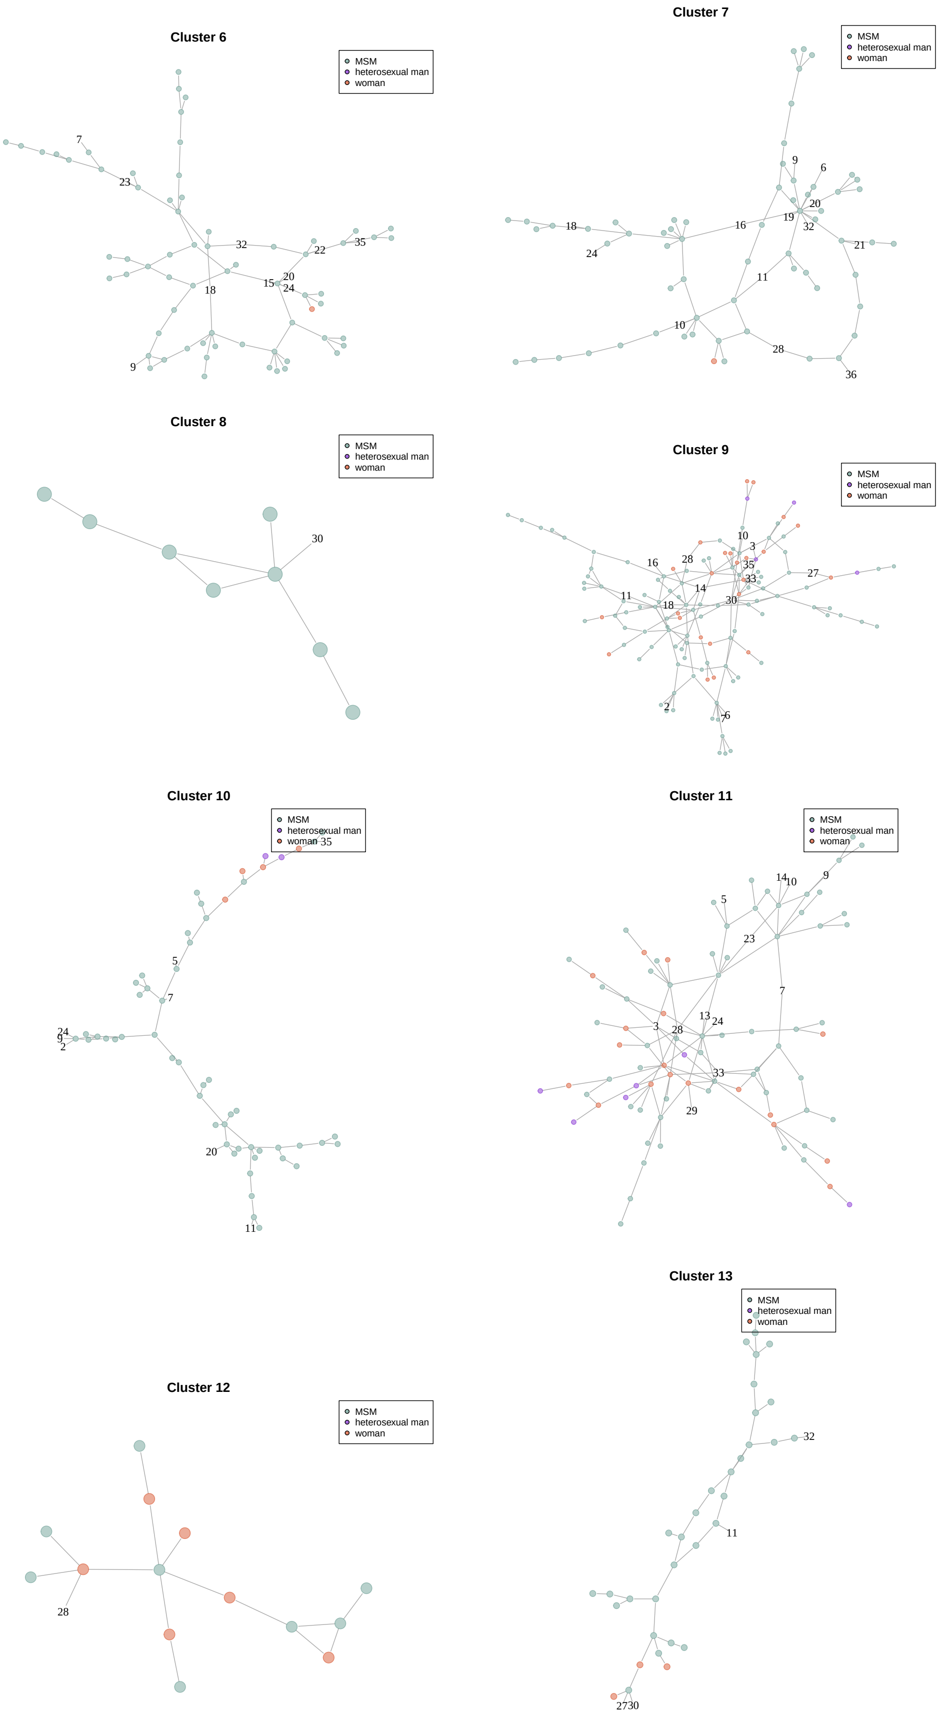


Figure 13: *Clusters from the largest connected components. Numbered nodes represent other clusters.*

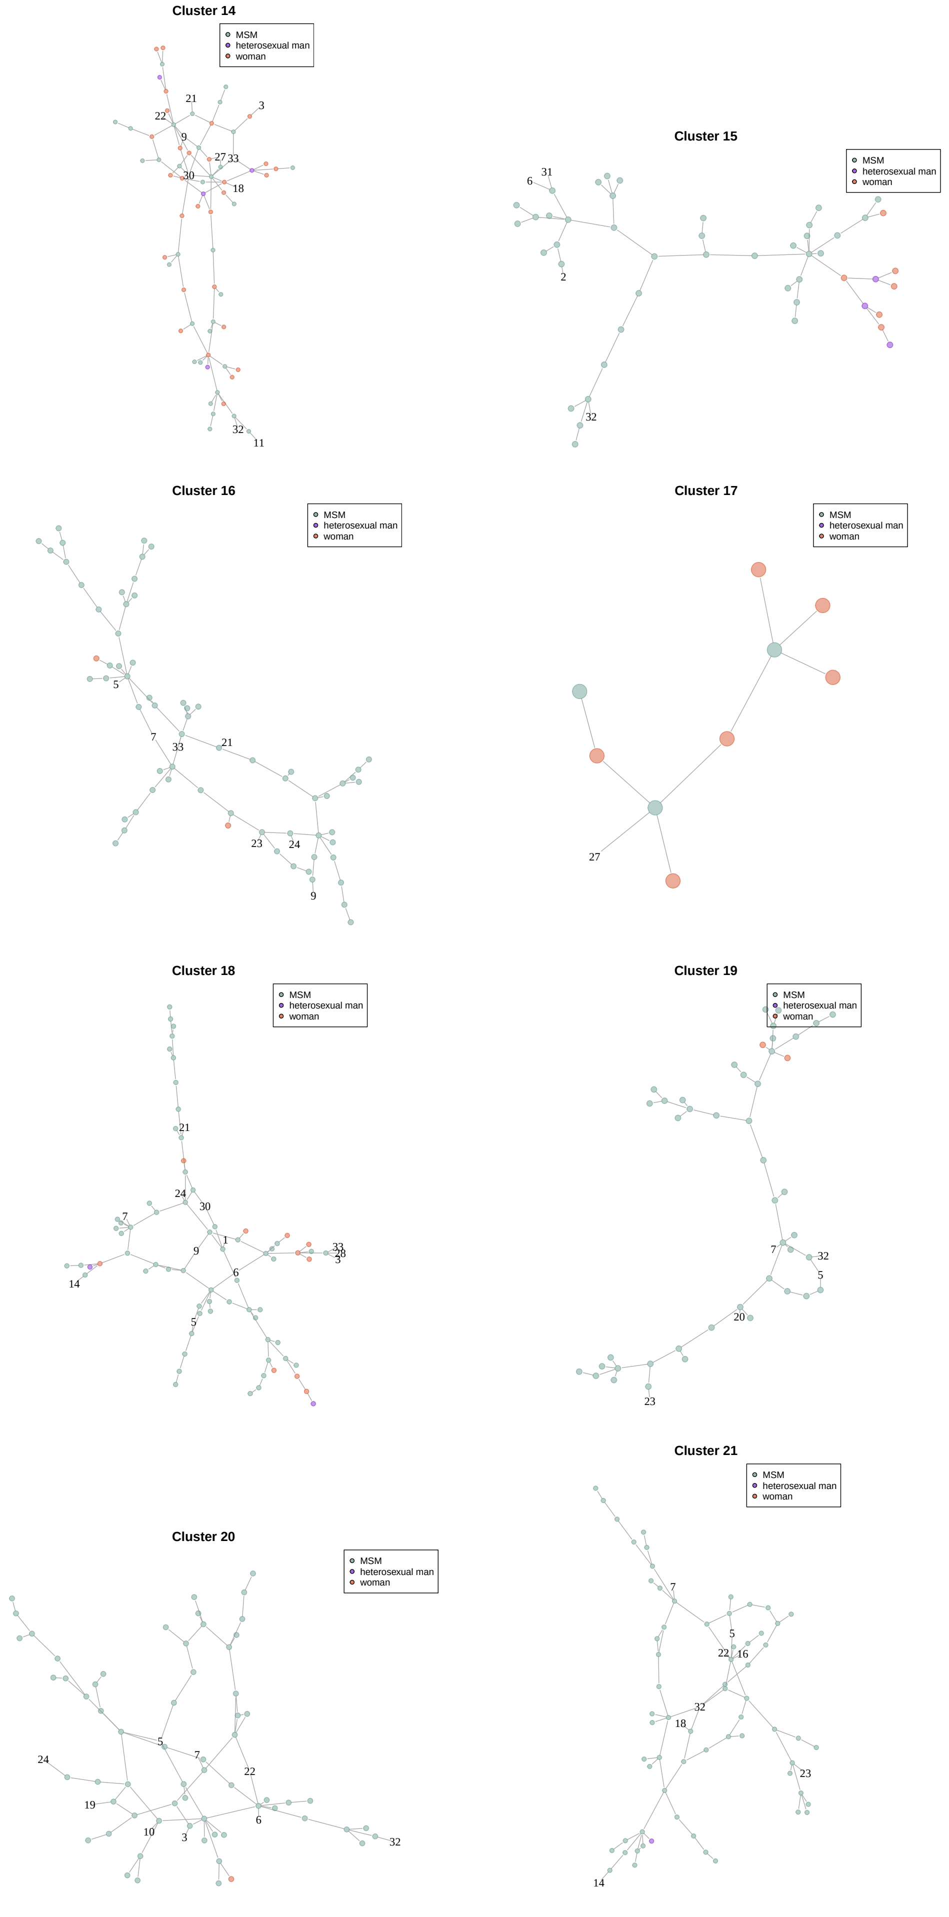


Figure 14: *Clusters from the largest connected components. Numbered nodes represent other clusters.*

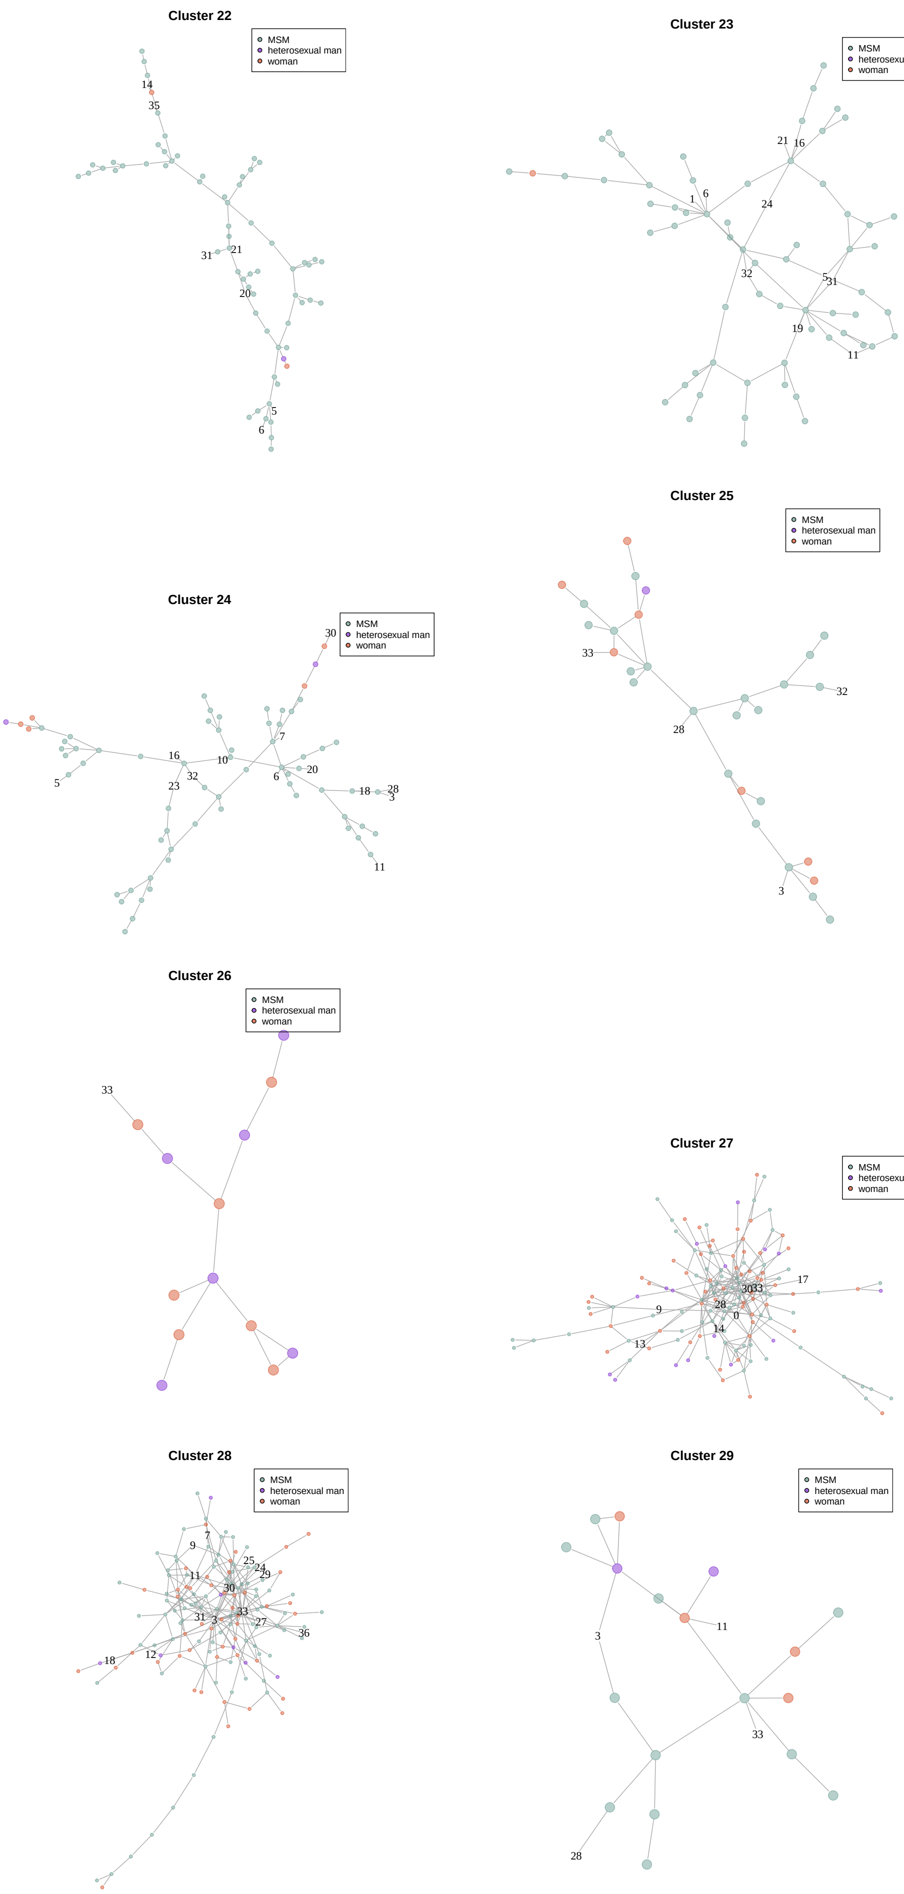


Figure 15: *Clusters from the largest connected components. Numbered nodes represent other clusters.*

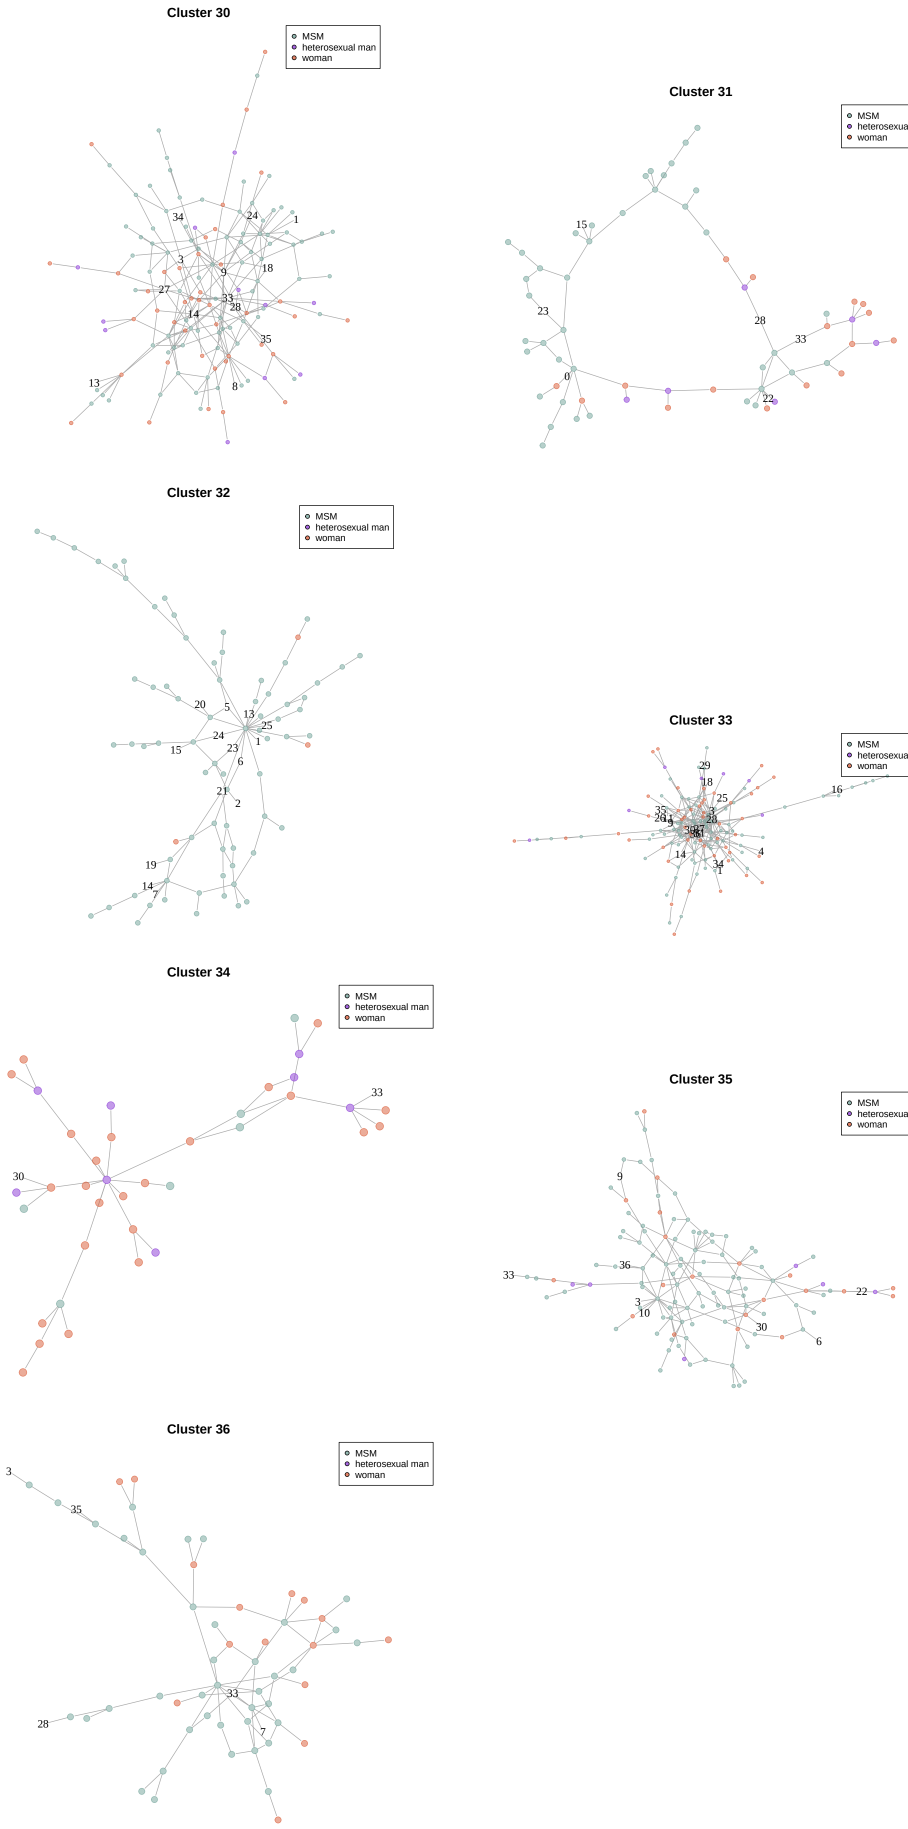


Figure 16: *Clusters from the largest connected components. Numbered nodes represent other clusters.*

# Acknowledgements

This work has been financed by ANR Viroscopy (ANR-08-SYSC-016-03), Chaire Mathématiques et Modélisation de la Biodiversité (Ec. Polytechnique, Museum National d'Histoire Naturelle et Fondation X), ANR MANEGE (ANR-09-BLAN-0215) and Labex CEMPI (ANR-11-LABX-0007-01). The authors thank Dr. J. Perez of the National Institute of Tropical Diseases in Cuba for granting access to the HIV/AIDS database.


# References


[1] A. Barrat and M. Weight. On the properties of 'small-world' networks. *Euro. Phys. J. B*, 13:547–560, 2000.

[2] M. Blum and V.C. Tran. HIV with contact-tracing: a case study in Approximate Bayesian Computation. *Biostatistics*, 11(4):644–660, 2010.

[3] S. Clémençon, H. De Arazoza, F. Rossi, and V.C. Tran. Visual mining of epidemic networks. In Joan Cabestany, Ignacio Rojas, and Gonzalo Joya, editors, *Advances in Computational Intelligence, Proceedings of 11th International Work-Conference on Artificial Neural Networks (IWANN 2011)*, number 6692 in Lecture Notes in Computer Science, pages 276–283. Springer Berlin / Heidelberg, Malaga, Spain, 2011.

[4] S. Clémençon, H. De Arazoza, F. Rossi, and V.C. Tran. A network analysis of the HIV-AIDS epidemics in Cuba. *Social Network Analysis and Mining*, 2015. main article.

[5] S. Clémençon, V.C. Tran, and H. De Arazoza. A stochastic SIR model with contact-tracing: large population limits and statistical inference. *Journal of Biological Dynamics*, 2(4):391–414, 2008.

[6] K.I. Goh, E. Oh, H. Jeong, B. Kahng, and D. Kim. Classification of scale-free networks. *Proc. Natl. Acad. Sci. USA*, 99:12583–12588, 2002.

[7] Y.-H. Hsieh, Y.-S. Wang, H. De Arazoza, and R. Lounes. Modeling secondary level of HIV contact tracing: its impact on HIV intervention in Cuba. *BMC Infectious Diseases 2010, 10:194*, 10:194, 2010.

[8] Michael Molloy and Bruce Reed. A critical point for random graphs with a given degree sequence. *Random Struct. Algorithms*, 6(2/3):161–179, 1995.

[9] M.E.J Newman. The structure and function of complex networks. *SIAM Review*, 45:167–256, November 2003.

[10] R.B. Rothenberg, D.E. Woodhouse, J.J. Potterat, S.Q. Muth, W.W. Darrow, and A.S. Klovdahl. Social networks in disease transmission: The Colorado Springs study. In R.H Needle, S.L. Coyle, S.G. Genser, and R.T. Trotter II, editors, *Social networks, drug abuse and HIV transmission*, volume 151 of *Research Monographs*, pages 3–18. National Instit, 1995.

[11] D.J. Watts and S.H. Strogatz. Collective dynamics of small-world networks. *Nature*, 393:440–442, 1998.

[12] J.L. Wylie and A. Jolly. Patterns of Chlamydia and Gonorrhea infection in sexual networks in Manitoba, Canada. *Sexually transmitted diseases*, 28(1):14–24, January 2001.
